# Supplementary material for: Regression-based causal inference with factorial experiments: estimands, model specifications, and design-based properties
Source: arXiv:2101.02400 source file (2021-12-08)
Supplement: Supplementary file 1 [file Biometrika_supp_20211111_final.pdf]

*Biometrika* (2021), **xx**, x, *pp.* 1–29
*Printed in Great Britain*

# Supplementary material for "Regression-based causal inference with factorial experiments: estimands, model specifications, and design-based properties"

BY ANQI ZHAO

*Department of Statistics and Data Science, National University of Singapore, 117546, Singapore*

staza@nus.edu.sg

AND PENG DING

*Department of Statistics, University of California, 425 Evans Hall, Berkeley, California 94720, U.S.A.*

pengdingpku@berkeley.edu

The Supplementary Material proceeds as follows.

- §A states the general theory for the $Q_1 \times \cdots \times Q_K$ factorial experiment. Although some parts of §A replicate those in §5 of the main text, we keep them to make §A self-contained.
- §B gives the proofs of the results under the $Q_1 \times \cdots \times Q_K$ factorial experiment, which imply those under the $2^2$, $2^3$, and $2^K$ experiments as special cases.
- §C gives more details for the special cases and includes some additional results on the analysis of variance and the HC2 correction of the robust covariance.
- §D presents the simulation studies and an empirical example.

We use the following notation below. For a vector $x$, let $\|x\|_1$ denote its $L_1$-norm; let $\|x\|_0$ denote its $L_0$-norm, i.e., the number of nonzero coordinates in $x$; let $\text{sgn}(x) = (-1)^{\|x\|_0}$. All vectors are assumed to be column vectors unless stated otherwise.

For positive integers $n$ and $l$, let $1_n$ and $0_n$ be the $n \times 1$ vectors of ones and zeros, let $0_{n\times l}$ be the $n \times l$ matrix of zeros, let $J_n$ be the $n \times n$ matrix of ones, and let $I_n$ be the $n \times n$ identity matrix, respectively. We suppress the dimensions in the subscripts when no confusion would arise. For an arbitrary set of real numbers $\{u_s : s \in \mathcal{S}\}$, let $\text{diag}(u_s) = \text{diag}(u_s)_{s\in\mathcal{S}}$ be the $|\mathcal{S}| \times |\mathcal{S}|$ diagonal matrix with $(u_s)_{s\in\mathcal{S}}$ on the diagonal. In particular, $\text{diag}(u_z) = \text{diag}(u_z)_{z\in\mathcal{T}}$ denotes the $Q \times Q$ diagonal matrix with $\{u_z : z \in \mathcal{T}\}$ on the diagonal; $\text{diag}(u_i) = \text{diag}(u_i)_{i=1}^N$ denotes the $N \times N$ diagonal matrix with $(u_i)_{i=1}^N$ on the diagonal. For an arbitrary matrix $M$, let $M_{[-1,]}$ denote the submatrix of $M$ without the first row. Let $\otimes$ denote the Kronecker product of matrices.

With a slight abuse of notation, we will also use $0_k$ and $1_k$ to denote the levels 0 and 1 of factor $k$ in the $Q_1 \times \cdots \times Q_K$ experiment when multiple factors are involved; the precise meaning will be made clear in the context.

We use "$\star$" to denote a part of the mathematical expressions that does not affect the proof.

## A. A GENERAL THEORY FOR THE $Q_1 \times \cdots \times Q_K$ FACTORIAL EXPERIMENT.

The $Q_1 \times \cdots \times Q_K$ factorial experiment features $K$ factors of interest, $k = 1, \ldots, K$, each of $Q_k \geq 2$ levels, indexed by $z_k \in \mathcal{F}_k = \{0, \ldots, Q_k - 1\}$. The $Q = \prod_{k=1}^K Q_k$ treatment combinations consist of $\mathcal{T} = \{z = (z_1, \ldots, z_K) : z_k \in \mathcal{F}_k,\ k = 1, \ldots, K\}$. Let $Z_{ik} \in \mathcal{F}_k$ denote the level of factor $k$ received

© 2018 Biometrika Trust

by unit $i$, with $Z_i = (Z_{i1}, \dots, Z_{iK})$. The canonical factor-based regression takes the form

$$Y_i \sim \prod_{k=1}^{K} \left\{ 1 + \sum_{z_k=1}^{Q_k-1} \mathcal{I}(Z_{ik} = z_k) \right\}, \tag{A1}$$

regressing $Y_i$ on the factor indicators $\mathcal{I}(Z_{ik} = z_k)$ and their products. Of interest is the utility of this regression and its variants for inferring causal effects from the design-based perspective.

Let $\mathcal{K}$ be a non-empty subset of $[K]$, taking values from $\mathcal{P}_K = \{\mathcal{K} : \emptyset \neq \mathcal{K} \subseteq [K]\}$. Let $z_{\mathcal{K}} = (z_k)_{k\in\mathcal{K}}$ and $z_{\overline{\mathcal{K}}} = (z_k)_{k\notin\mathcal{K}}$ index the combinations of factors in $\mathcal{K}$ and $\overline{\mathcal{K}} = [K]\backslash\mathcal{K}$, respectively, taking values from $\mathcal{F}_{\mathcal{K}} = \prod_{k\in\mathcal{K}} \mathcal{F}_k$ and $\mathcal{F}_{\overline{\mathcal{K}}} = \prod_{k\notin\mathcal{K}} \mathcal{F}_k$. In particular, $z_{[K]} = z \in \mathcal{T}$ and $\mathcal{F}_{[K]} = \mathcal{T}$. Let $Z_{i,\mathcal{K}} = (Z_{ik})_{k\in\mathcal{K}}$ and $Z_{i,\overline{\mathcal{K}}} = (Z_{ik})_{k\notin\mathcal{K}}$ with $Z_{i,[K]} = Z_i$.

Let $0_k$ be the baseline level of factor $k$, and let $\mathcal{F}_k^* = \mathcal{F}_k\backslash\{0_k\}$ be the set of the non-baseline levels, indexed by $z_k^*$. As a convention, we use the superscript "$*$" to signify non-baseline levels. Let $\mathcal{F}_{\mathcal{K}}^* = \prod_{k\in\mathcal{K}} \mathcal{F}_k^*$ be a subset of $\mathcal{F}_{\mathcal{K}}$, consisting of $z_{\mathcal{K}}^* = (z_k^*)_{k\in\mathcal{K}}$ with non-baseline levels in all dimensions. Let $\mathcal{F}^* = \cup_{\mathcal{K}\in\mathcal{P}_K} \mathcal{F}_{\mathcal{K}}^*$ be the collection of $z_{\mathcal{K}}^*$ over all non-empty $\mathcal{K}$. Then (A1) equals

$$Y_i \sim 1 + \sum_{\mathcal{K}\in\mathcal{P}_K} \sum_{z_{\mathcal{K}}^*\in\mathcal{F}_{\mathcal{K}}^*} \prod_{k\in\mathcal{K}} \mathcal{I}(Z_{ik} = z_k^*) \sim 1 + \sum_{z_{\mathcal{K}}^*\in\mathcal{F}^*} \prod_{k\in\mathcal{K}} \mathcal{I}(Z_{ik} = z_k^*).$$

Consider $K$ types of factorial effects, quantifying the main effects and two- to $K$-way interactions of the factors of interest, respectively. Refer to them interchangeably as the first- to $K$th-order factorial effects, respectively. We first define the conditional factorial effects by induction in §A.1, and then define the general factorial effects as their respective weighted averages in §A.2.

### A.1. *Definition of the conditional factorial effects*

As a general rule, we define by induction the $m$th-order conditional factorial effect as the difference between two $(m-1)$th-order conditional effects for $m = 2, \dots, K$. For notational simplicity, we illustrate the definition of the $m$th-order effects using the first $m$ factors with $\mathcal{K} = [m]$ and

$$z_{[m]}^* = (z_k^*)_{k=1}^m, \quad \mathcal{F}_{[m]}^* = \prod_{k=1}^m \mathcal{F}_k^*, \quad z_{(m+1):K} = (z_k)_{k=m+1}^K, \quad \mathcal{F}_{(m+1):K} = \prod_{k=m+1}^K \mathcal{F}_k.$$

DEFINITION A1. *Let $\bar{Y}(z_1, z_{2:K})$ be the average potential outcome under $z = (z_1, z_{2:K}) \in \mathcal{T}$, and define $\tau(z_1^* \mid z_{2:K}) = \bar{Y}(z_1^*, z_{2:K}) - \bar{Y}(0_1, z_{2:K})$ as the conditional effect of factor 1 at level $z_1^* \in \mathcal{F}_1^*$ when factors 2 to $K$ are fixed at $z_{2:K} \in \mathcal{F}_{2:K}$.*

*Given $\tau(z_{[m-1]}^* \mid z_{m:K})$ as the conditional $(m-1)$th-order factorial effect of factors 1 to $(m-1)$ at level $z_{[m-1]}^* \in \mathcal{F}_{[m-1]}^*$ when the rest of the factors are fixed at $z_{m:K} \in \mathcal{F}_{m:K}$ for $m = 2, \dots, K-1$, define*

$$\tau(z_{[m]}^* \mid z_{(m+1):K}) = \tau(z_{[m-1]}^* \mid z_m^*, z_{(m+1):K}) - \tau(z_{[m-1]}^* \mid 0_m, z_{(m+1):K})$$

*as the conditional $m$th-order factorial effect of factors 1 to $m$ at level $z_{[m]}^* = (z_{[m-1]}^*, z_m^*) \in \mathcal{F}_{[m]}^*$ when the rest of the factors are fixed at $z_{(m+1):K} \in \mathcal{F}_{(m+1):K}$.*

*For $m = K$, define $\tau(z^*) = \tau(z_{[K]}^*) = \tau(z_{[K-1]}^* \mid z_K^*) - \tau(z_{[K-1]}^* \mid 0_K)$ as the $K$-way interaction of factors 1 to $K$ at level $z^* \in \mathcal{T}$.*

Definition A1 formalizes the $m$th-order conditional effect of combination $z_{[m]}^*$ as the difference between two $(m-1)$th-order conditional effects of combination $z_{[m-1]}^*$ when the level of factor $m$ changes from $0_m$ to $z_m^* \in \mathcal{F}_m^*$. We can obtain the explicit form of $\tau(z_{[m]}^* \mid z_{(m+1):K})$ in terms of the average potential outcomes, which further ensures that the order in which new factors are added to the combination in the induction does not matter. See Lemma B3 for details.

The definition extends to general $\mathcal{K}$ by symmetry. Denote by $\tau(z_{\mathcal{K}}^* \mid z_{\overline{\mathcal{K}}})$ the conditional $|\mathcal{K}|$-th order factorial effect of factors in $\mathcal{K}$ at non-baseline level $z_{\mathcal{K}}^* \in \mathcal{F}_{\mathcal{K}}^*$ when the rest of the factors are fixed at $z_{\overline{\mathcal{K}}} \in \mathcal{F}_{\overline{\mathcal{K}}}$. This gives a total of $|\mathcal{F}_{\mathcal{K}}^*| \times |\mathcal{F}_{\overline{\mathcal{K}}}|$ conditional factorial effects for the $|\mathcal{K}|$ factors in a fixed $\mathcal{K}$. As a

special case, the $2^K$ experiment features $\mathcal{F}_k = \{0_k, 1_k\}$ such that $\mathcal{F}^*_{\mathcal{K}}$ consists of only one element, namely $1_{\mathcal{K}} = (1_k)_{k\in\mathcal{K}}$, for all $\mathcal{K} \in \mathcal{P}_K$. This ensures a one-to-one mapping between $\mathcal{K}$ and $1_{\mathcal{K}}$, and reconciles the notation from the $2^K$ case with Definition A1 as $\tau_{\mathcal{K}}(z_{\overline{\mathcal{K}}}) = \tau(1_{\mathcal{K}} \mid z_{\overline{\mathcal{K}}})$.

### A.2. *Definition of the general factorial effects*

We next define the general factorial effects as weighted averages of their respective conditional counterparts. Let $\pi_{\mathcal{K}} = \{\pi(z_{\mathcal{K}}) : z_{\mathcal{K}} \in \mathcal{F}_{\mathcal{K}}\}$ denote a weighting vector over the $|\mathcal{F}_{\mathcal{K}}| = \prod_{k\in\mathcal{K}} Q_k$ possible values of $z_{\mathcal{K}} \in \mathcal{F}_{\mathcal{K}}$, and let $\pi = \{\pi_{\mathcal{K}} : \mathcal{K} \in \mathcal{P}_K\}$ denote the weighting scheme that summarizes $\pi_{\mathcal{K}}$ over all non-empty $\mathcal{K}$.

DEFINITION A2. *Given conditional factorial effects $\tau(z^*_{\mathcal{K}} \mid z_{\overline{\mathcal{K}}})$ from Definition A1 for all non-empty $\mathcal{K} \subseteq [K]$ and $(z^*_{\mathcal{K}}, z_{\overline{\mathcal{K}}}) \in \mathcal{F}^*_{\mathcal{K}} \times \mathcal{F}_{\overline{\mathcal{K}}}$, define $\tau_\pi(z^*_{\mathcal{K}}) = \sum_{z_{\overline{\mathcal{K}}}\in\mathcal{F}_{\overline{\mathcal{K}}}} \pi(z_{\overline{\mathcal{K}}}) \cdot \tau(z^*_{\mathcal{K}} \mid z_{\overline{\mathcal{K}}})$ as the general factorial effect of factors in $\mathcal{K}$ at level $z^*_{\mathcal{K}}$ under weighting scheme $\pi$.*

Definitions A1 and A2 together complete the definition of the $(Q-1)$ general factorial effects, vectorized as

$$\tau_\pi = \{\tau_\pi(z^*_{\mathcal{K}}) : z^*_{\mathcal{K}} \in \mathcal{F}^*\} = G_\pi \bar{Y}.$$

Refer to $\tau_\pi(z^*_{\mathcal{K}})$ as the standard effect if $\pi(z_{\overline{\mathcal{K}}}) = |\mathcal{F}_{\overline{\mathcal{K}}}|^{-1}$ are identical for all $z_{\overline{\mathcal{K}}} \in \mathcal{F}_{\overline{\mathcal{K}}}$. Refer to $\tau_\pi(z^*_{\mathcal{K}})$ as the empirical effect if $\pi(z_{\overline{\mathcal{K}}}) = N^{-1}\sum_{i=1}^N \mathcal{I}(Z_{i,\overline{\mathcal{K}}} = z_{\overline{\mathcal{K}}})$ equals the empirical proportion in the actual experiment.

We further restrict the discussion to coherent weighting schemes in Definition A3 below as a natural extension of Definition 2. A coherent weighting scheme intuitively corresponds to a distribution over $\mathcal{T}$.

DEFINITION A3. *The weighting vector $\pi_{[K]} = \{\pi(z) : z \in \mathcal{T}\}$ in $\pi$ defines a distribution over $\mathcal{T}$, represented by $\pi(z) = \mathrm{pr}(Z = z) = \mathrm{pr}(Z_1 = z_1, \ldots, Z_K = z_K)$. A weighting scheme $\pi$ is coherent if for all $\mathcal{K} \in \mathcal{P}_K$, the weighting vector $\pi_{\mathcal{K}} = \{\pi(z_{\mathcal{K}}) : z_{\mathcal{K}} \in \mathcal{F}_{\mathcal{K}}\}$ equals the distribution of $Z_{\mathcal{K}} = (Z_k)_{k\in\mathcal{K}}$ under $\{\pi(z) : z \in \mathcal{T}\}$; that is, $\pi(z_{\mathcal{K}}) = \mathrm{pr}(Z_{\mathcal{K}} = z_{\mathcal{K}}) = \sum_{z_{\overline{\mathcal{K}}}\in\mathcal{F}_{\overline{\mathcal{K}}}} \pi(z_{\mathcal{K}}, z_{\overline{\mathcal{K}}})$ for all $\mathcal{K} \in \mathcal{P}_K$.*

### A.3. *Factor-based regression with the saturated model*

For prespecified $\delta = \{\delta_k(z^*_k) : k \in [K],\ z^*_k \in \mathcal{F}^*_k\}$ with $0 \le \delta_k(z^*_k) \le 1$ and $0 \le \sum_{z^*_k\in\mathcal{F}^*_k} \delta_k(z^*_k) \le 1$, the regression (5) from the $2^K$ case motivates the location-shift transformation $\mathcal{I}_\delta(Z_{ik} = z^*_k) = \mathcal{I}(Z_{ik} = z^*_k) - \delta_k(z^*_k)$ and the corresponding saturated regression

$$Y_i \sim 1 + \sum_{z^*_{\mathcal{K}}\in\mathcal{F}^*} f_i(z^*_{\mathcal{K}}), \tag{A2}$$

where $f_i(z^*_{\mathcal{K}}) = \prod_{k\in\mathcal{K}} \mathcal{I}_\delta(Z_{ik} = z^*_k)$. Let $\hat\gamma$ and $\hat\Psi$ be the coefficient vector and robust covariance of the $(Q-1)$ non-intercept terms in (A2), respectively, with elements arranged in the same order of $z^*_{\mathcal{K}}$ as those in $\tau_\pi$. We derive below their utility for the Wald-type inference of $\tau_\pi$.

The notion of product weighting scheme extends naturally to the current setting as $\pi(z) = \prod_{k=1}^K \pi(z_k)$ for all $z \in \mathcal{T}$, and is fully determined by the values of $\{\pi(z^*_k) : z^*_k \in \mathcal{F}^*_k\}_{k=1}^K$. The standard effects satisfy the product structure whereas the empirical effects may not. Building on the intuition from the $2^K$ experiment, Definition A4 introduces two product weighting schemes of particular importance, arising from the estimand of interest and the location-shift parameters, respectively.

DEFINITION A4. *For an arbitrary weighting scheme $\pi$, let $\pi_\times$ be the product weighting scheme with $\pi_\times(z^*_k) = \pi(z^*_k)$ for all $k = 1, \ldots, K$ and $z^*_k \in \mathcal{F}^*_k$.*

*For arbitrary location-shift parameters $\delta$ with $0 \le \delta_k(z^*_k) \le 1$ and $0 \le \sum_{z^*_k\in\mathcal{F}^*_k} \delta_k(z^*_k) \le 1$, let $\delta_\times$ be the product weighting scheme with $\delta_\times(z^*_k) = \delta_k(z^*_k)$ for all $k = 1, \ldots, K$ and $z^*_k \in \mathcal{F}^*_k$.*

The product weighting scheme $\pi_\times$ satisfies $\pi_\times = \pi$ if $\pi$ is already a product weighting scheme. Let $\tau_{\delta\times} = G_{\delta\times}\bar{Y}$ be the vector of general factorial effects under weighting scheme $\delta_\times$, $\hat\tau_{\delta\times} = G_{\delta\times}\hat{Y}$ be its moment estimator, and $\hat{\mathrm{cov}}(\hat\tau_{\delta\times}) = G_{\delta\times}\hat{V}G^{\mathrm{T}}_{\delta\times}$ be the estimated covariance, respectively. Theorems A1

and A2 generalize Theorems 1 and 2 in the main text, and justify the use of (A2) for inferring $\tau_\pi$ under product and general coherent weighting schemes, respectively.

THEOREM A1. *Under the $Q_1 \times \cdots \times Q_K$ experiment, the outputs of* (A2) *satisfy* $\hat{\gamma} = \hat{\tau}_{\delta\times}$ *and* $\hat{\Psi} = \widehat{\mathrm{cov}}(\hat{\tau}_{\delta\times}) - G_{\delta\times}\,\mathrm{diag}(N_z^{-1})\hat{V}G_{\delta\times}^{\mathrm{T}}$.

*Condition A*1. Assume $\tau(z^*_{\mathcal{K}} \mid z_{\overline{\mathcal{K}}}) = 0$ for all $z^*_{\mathcal{K}}$ and $z_{\overline{\mathcal{K}}}$ with $|\mathcal{K}| = 3$.

Condition A1 rules out the existence of three-way interactions and thus that of all $m$-way interactions for $3 < m \leq K$ by Definition A1. We will refer to it as the no three-way interactions condition hence for simplicity.

THEOREM A2. *Under the $Q_1 \times \cdots \times Q_K$ experiment and Condition A*1*, we have $\tau_\pi = \tau_{\pi\times}$ for all coherent $\pi$, where $\tau_\pi$ and $\tau_{\pi\times}$ are the vectors of general factorial effects under $\pi$ and $\pi_\times$, respectively.*

The Wald-type inference of $\tau_\pi$ can thus be conducted via (A2) with $\delta_k(z^*_k)$ set at $\pi(z^*_k)$ for all coherent $\pi$ in the absence of three-way interactions. The proof of Theorem A2 further shows that the requirement of $\tau(z^*_{\mathcal{K}} \mid z_{\overline{\mathcal{K}}}) = 0$ for all $|\mathcal{K}| = 3$ is not only sufficient but also necessary for $\tau_\pi = \tau_{\pi\times}$ to hold if $\pi$ is coherent but not a product weighting scheme.

### A.4. *Factor-based regression with unsaturated models*

We next consider

$$Y_i \sim 1 + \sum_{z^*_{\mathcal{K}} \in \mathcal{F}_+} f_i(z^*_{\mathcal{K}}), \tag{A3}$$

where $\mathcal{F}_+ \subset \mathcal{F}^*$, as an unsaturated variant of (A2) when only a subset of the $(Q-1)$ factorial effects are of interest, vectorized as $\tau_{\pi,+} = \{\tau_\pi(z^*_{\mathcal{K}}) : z^*_{\mathcal{K}} \in \mathcal{F}_+\}$. Let $\tilde{\gamma}_+$ and $\tilde{\Psi}_+$ be the coefficient vector and robust covariance of the $|\mathcal{F}_+|$ non-intercept terms in (A3), respectively. We establish in this section their utility for inferring $\tau_{\pi,+}$.

Recall $\hat{\gamma}$ as the coefficient vector of the non-intercept terms from (A2). Partition it into $\hat{\gamma}_+$ and $\hat{\gamma}_-$, corresponding to the coefficients of $\{f_i(z^*_{\mathcal{K}})\}_{z^*_{\mathcal{K}} \in \mathcal{F}_+}$ and $\{f_i(z^*_{\mathcal{K}})\}_{z^*_{\mathcal{K}} \notin \mathcal{F}_+}$, respectively. As a convention, we use "+" and "−" in the subscripts to signify effects included in and omitted from the unsaturated regression (A3), respectively. Inherit all the other notation from §5.5 in the main text with $P_N = I_N - N^{-1}J_N$ and $Y = (Y_1, \ldots, Y_N)^{\mathrm{T}}$. Theorem A3 below extends Theorem 3 and gives the numeric correspondence between $\tilde{\gamma}_+$ and $\hat{\gamma}$.

THEOREM A3. *Under the $Q_1 \times \cdots \times Q_K$ experiment, the coefficients from* (A2) *and* (A3) *satisfy $\tilde{\gamma}_+ = \hat{\gamma}_+ + D\hat{\gamma}_-$ with $D\hat{\gamma}_- = 0$ if and only if $F^{\mathrm{T}}_{+[,-1]}P_N F_-(R^{\mathrm{T}}R)^{-1}R^{\mathrm{T}}Y = 0$. Two sufficient conditions for $D\hat{\gamma}_- = 0$ for all $Y$ are $F_+^{\mathrm{T}}F_- = 0$ or $F_+^{\mathrm{T}}P_N F_- = 0$.*

Recall that $\hat{\gamma}_+$ and $\hat{\gamma}_-$ coincide with the moment estimators of $\tau_{\delta\times,+} = \{\tau_{\delta\times}(z^*_{\mathcal{K}}) : z^*_{\mathcal{K}} \in \mathcal{F}_+\}$ and $\tau_{\delta\times,-} = \{\tau_{\delta\times}(z^*_{\mathcal{K}}) : z^*_{\mathcal{K}} \notin \mathcal{F}_+\}$, respectively, denoted by $\hat{\tau}_{\delta\times,+}$ and $\hat{\tau}_{\delta\times,-}$. Theorem A3 gives two sufficient conditions for $\tilde{\gamma}_+$ to recover the exact moment estimator $\hat{\tau}_{\delta\times,+}$, requiring orthogonality of $F_+$ and $F_-$ either in original form or after centered by the column averages. Corollary A1 below gives a sufficient condition for $F_+^{\mathrm{T}}F_- = 0$. The resulting regression targets standard factorial effects under the balanced design. Compare it with Corollary 1 to see the extra requirement on the composition of $\mathcal{F}_+$ under the general $Q_1 \times \cdots \times Q_K$ experiment.

COROLLARY A1. *Under the $Q_1 \times \cdots \times Q_K$ experiment, $\tilde{\gamma}_+ = \hat{\gamma}_+$ if* (i) $N_z = N/Q$ *for all $z \in \mathcal{T}$,* (ii) $\delta_k(z^*_k) = Q_k^{-1}$ *for all $k = 1, \ldots, K$ and $z^*_k \in \mathcal{F}^*_k$, and* (iii) *the elements in $\mathcal{F}^*_{\mathcal{K}}$ are either all included in the unsaturated specification, namely $\mathcal{F}^*_{\mathcal{K}} \subseteq \mathcal{F}_+$, or all excluded, namely $\mathcal{F}^*_{\mathcal{K}} \subseteq \mathcal{F}^* \backslash \mathcal{F}_+$, for all $\mathcal{K} \in \mathcal{P}_K$.*

Conditions (i) and (ii) stipulate the treatment sizes and the location-shift scheme, respectively; the qualified specifications are limited to those targeting the standard effects under balanced designs. Condition (iii) concerns the composition of $\mathcal{F}_+$. A special case is that $\mathcal{F}_+ = \cup_{\mathcal{K}:|\mathcal{K}| \leq m} \mathcal{F}^*_{\mathcal{K}}$, including up to $m$th-order terms for some $m \in [K]$.

Despite the loss of exact recovery of the moment estimator in general, Theorem A3 ensures that $\tilde{\gamma}_+$ is unbiased as long as the nuisance effects $\tau_{\delta_\times,-}$ are indeed zero.

*Condition A2.* The nuisance effects are zero, that is, $\tau_\pi(z^*_\mathcal{K}) = 0$ for all $z^*_\mathcal{K} \notin \mathcal{F}_+$.

THEOREM A4. *Under the completely randomized $Q_1 \times \cdots \times Q_K$ experiment, the coefficients from* (A3) *satisfy $E(\tilde{\gamma}_+) = \tau_{\delta_\times,+} + D\tau_{\delta_\times,-}$ and $\text{cov}(\tilde{\gamma}_+) = (I, D)G_{\delta_\times}\text{cov}(\hat{Y})G^{\mathrm{T}}_{\delta_\times}(I, D)^{\mathrm{T}}$. Further assume Condition* 1 *and Condition A2 with $\pi = \delta_\times$. Then $E(\tilde{\gamma}_+) = \tau_{\delta_\times,+}$, and $\tilde{\gamma}_+$ is asymptotically Normal with $N\{\tilde{\Psi}_+ - \text{cov}(\tilde{\gamma}_+)\} = \Delta + o_{\mathrm{p}}(1)$, where $\Delta = (I, D)G_{\delta_\times}SG^{\mathrm{T}}_{\delta_\times}(I, D)^{\mathrm{T}} \geq 0$.*

Theorem A4 justifies the Wald-type inference of $\tau_{\delta_\times,+}$ from the unsaturated specification (A3) when the nuisance effects omitted indeed do not exist. The resulting $\tilde{\gamma}_+$ is both unbiased and consistent for estimating $\tau_{\delta_\times,+}$, with the robust covariance $\tilde{\Psi}_+$ affording an asymptotically conservative estimator for the true sampling covariance. The proof of Theorem A1 further shows that the intercept from (A3) is an unbiased estimator of a weighted average of $\bar{Y}(z)$ instead of a contrast and is thus non-zero in general. This suggests the necessity to include the intercept in the unsaturated specification for the satisfaction of Condition A2. One limitation of (A3), again, lies in its requirement on the product weighting scheme. Juxtaposing Condition A1, Condition A2, and Theorem A2 together ensures that the result of Theorem A4 extends to $\tau_{\pi,+}$ for all coherent $\pi$ in the absence of three-way interactions.

Theorem A5 below extends Remark 2 and states the efficiency of $\tilde{\gamma}_+$ over $\hat{\gamma}_+$ under Condition 2.

THEOREM A5. *Under the completely randomized $Q_1 \times \cdots \times Q_K$ experiment and Condition* 2*,*

$$\text{cov}(\tilde{\gamma}_+) \leq \text{cov}(\hat{\gamma}_+) - s_0 D(R^{\mathrm{T}}R)^{-1}D^{\mathrm{T}} \leq \text{cov}(\hat{\gamma}_+),$$

*recalling that $R$ is the residual matrix from the column-wise regression of $F_-$ on $F_+$. Further assume Condition A2 with $\pi = \delta_\times$. Then $\tilde{\gamma}_+$ is the best linear unbiased estimator of the form $L\hat{Y}$. That is, $\tilde{\gamma}_+$ is unbiased for $\tau_{\delta_\times,+}$ with $\text{cov}(\tilde{\gamma}_+) \leq \text{cov}(L\hat{Y})$ for any linear estimator $L\hat{Y}$ that satisfies $E(L\hat{Y}) = \tau_{\delta_\times,+}$.*

Theorems A4 and A5 together establish the bias-variance trade-off between the saturated and unsaturated regressions from the design-based perspective. Further, Theorem A5 gives a novel design-based Gauss–Markov theorem, ensuring that the unsaturated regression yields the best linear unbiased estimator under Conditions 2 and A2. As a sanity check, both $\tilde{\gamma}_+$ and $\hat{\gamma}_+$ have the form $L\hat{Y}$ and unbiasedly estimate $\tau_{\delta_\times,+}$ under Condition A2 with $\pi = \delta_\times$. The constant treatment effects condition is crucial for $\text{cov}(\tilde{\gamma}_+) \leq \text{cov}(\hat{\gamma}_+)$ to hold in Theorem A5. We give a counterexample below in the absence of it.

*Example A1.* Consider a $2^2$ factorial experiment with $(N_{00}, N_{01}, N_{10}, N_{11}) = (40, 30, 20, 10)$. We generate the potential outcomes $\{Y_i(z) : i = 1, \ldots, N;\ z \in \mathcal{T}\}$ as independent and identically distributed standard Normal random variables. For a particular configuration, we have

$$\text{cov}(\hat{Y}) = \text{diag}\{S(z,z)/N_z\}_{z\in\mathcal{T}} - N^{-1}S = \begin{pmatrix} 1.712 & -0.063 & -0.077 & 0.013 \\ -0.063 & 2.703 & -0.173 & -0.055 \\ -0.077 & -0.173 & 4.941 & 0.128 \\ 0.013 & -0.055 & 0.128 & 5.622 \end{pmatrix}.$$

Consider $Y_i \sim 1 + A'_i + B'_i + A'_iB'_i$ and $Y_i \sim 1 + A'_i + B'_i$ with $A'_i = A_i - 1/2$ and $B'_i = B_i - 1/2$ for estimating the standard main effects $\tau_{\mathrm{A}}$ and $\tau_{\mathrm{B}}$. Direct algebra shows

$$\text{cov}(\hat{\gamma}_+) = \begin{pmatrix} 3.923 & -0.171 \\ -0.171 & 3.726 \end{pmatrix}, \quad \text{cov}(\tilde{\gamma}_+) = \begin{pmatrix} 3.985 & -0.298 \\ -0.298 & 3.173 \end{pmatrix}.$$

With $3.923 < 3.985$, the coefficient of $A'_i$ from the saturated regression has a smaller variance than that from the unsaturated counterpart.

## A.5. *Weighted least squares*

Recall from Corollary A1 that orthogonality and balancedness together allow us to recover the moment estimators of the standard effects from unsaturated regressions even when the excluded nuisance effects

are not zero. We now show that the use of weighted least squares can further relax the requirement on balancedness, echoing the comment after Corollary 1 in the main paper.

Assume the weights for least squares fitting are identical for all units under the same treatment, denoted by $w_i = w(Z_i)$ for $i = 1, \dots, N$ and $Z_i \in \mathcal{T}$. The resulting weighted least squares fit yields identical estimators as the ordinary least squares fit under the saturated specification, yet opens the possibility to recover the standard effects directly from the unsaturated specifications even when the design is not balanced and the nuisance effects omitted are not zero. We formalize the intuition in Proposition A1 below. Recall $\hat{\gamma}$ and $\hat{\gamma}_+$ as the ordinary least squares coefficient vectors from the saturated regression (A2), corresponding to $\tau_\pi$ and $\tau_{\pi,+}$, respectively. Let $w(z)$ be the common value of $w_i$ for all $i$'s under treatment $z$. Let $\hat{\gamma}_{\text{wls}}$ and $\tilde{\gamma}_{\text{wls},+}$ be the corresponding weighted least squares coefficient vectors of the non-intercept terms from (A2) and (A3), respectively.

PROPOSITION A1. *Consider the $Q_1 \times \cdots \times Q_K$ experiment with $N_z > 0$ for $z \in \mathcal{T}$. With the saturated regression, $\hat{\gamma}_{\text{wls}} = \hat{\gamma}$. With the unsaturated regression, $\tilde{\gamma}_{\text{wls},+} = \tilde{\gamma}_+$ if* (i) *$w(z) \propto e_z^{-1}$ for $z \in \mathcal{T}$,* (ii) *$\delta_k(z_k^*) = Q_k^{-1}$ for all $k = 1, \dots, K$ and $z_k^* \in \mathcal{F}_k^*$, and* (iii) *the elements in $\mathcal{F}_\mathcal{K}^*$ are either all included in the unsaturated specification, namely $\mathcal{F}_\mathcal{K}^* \subseteq \mathcal{F}_+$, or all excluded, namely $\mathcal{F}_\mathcal{K}^* \subseteq \mathcal{F}^* \backslash \mathcal{F}_+$, for all $\mathcal{K} \in \mathcal{P}_K$.*

Compare Proposition A1 with Corollary A1. Weighted least squares with the inverse of treatment probability relaxes the requirement on balancedness for inference from unsaturated regressions, and recovers the moment estimators of the standard effects as long as the location-shift parameters are set accordingly and the elements in $\mathcal{F}_\mathcal{K}^*$ are either all included in the unsaturated specification or all excluded for all $\mathcal{K} \in \mathcal{P}_K$.

A natural question is the choice between ordinary and weighted least squares. On the one hand, Proposition A1 demonstrates the advantage of weighted least squares in unbalanced designs because with an unsaturated specification, $\tilde{\gamma}_{\text{wls},+}$ can still deliver unbiased estimators for the standard factorial effects whereas $\tilde{\gamma}_+$ in general can not. On the other hand, the design-based Gauss–Markov theorem implies that $\tilde{\gamma}_{\text{wls},+}$ is less efficient than $\tilde{\gamma}_+$ under the constant treatment effects condition. Therefore, the advantage of weighted least squares comes at the cost of efficiency.

## B. PROOFS OF THE RESULTS UNDER THE $Q_1 \times \cdots \times Q_K$ EXPERIMENT

### B.1. *Lemmas from the theory of least squares*

We review in this subsection some useful results from the theory of least squares. The proofs follow from direct algebra and are thus omitted.

For $X = (X_1, X_2)$ where $X_k$ is an $N \times L_k$ matrix for $k = 1, 2$, the inverse of the Gram matrix equals

$$(X^{\mathrm{T}}X)^{-1} = \left(\begin{array}{c|c} (X_1^{\mathrm{T}}X_1)^{-1} + \Phi(R^{\mathrm{T}}R)^{-1}\Phi^{\mathrm{T}} & -\Phi(R^{\mathrm{T}}R)^{-1} \\ \hline -(R^{\mathrm{T}}R)^{-1}\Phi^{\mathrm{T}} & (R^{\mathrm{T}}R)^{-1} \end{array}\right), \tag{B1}$$

where $\Phi = (X_1^{\mathrm{T}}X_1)^{-1}X_1^{\mathrm{T}}X_2$ and $R = X_2 - X_1\Phi$.

The following lemma states the invariance of least squares to non-degenerate linear transformation of the design matrix.

LEMMA B1. *Consider an $N \times 1$ vector $Y$ and two $N \times Q$ matrices, $X_1$ and $X_2$, that satisfy $X_2 = X_1\Gamma$ for some invertible $Q \times Q$ matrix $\Gamma$. The regressions*

$$Y = X_1\hat{\beta}_1 + \hat{\epsilon}_1, \quad Y = X_2\hat{\beta}_2 + \hat{\epsilon}_2$$

*yield robust covariances $\hat{\Psi}_1$ and $\hat{\Psi}_2$. They satisfy*

$$\hat{\beta}_1 = \Gamma\hat{\beta}_2, \quad \hat{\epsilon}_1 = \hat{\epsilon}_2, \quad \hat{\Psi}_1 = \Gamma\hat{\Psi}_2\Gamma^{\mathrm{T}}.$$

The following lemma reviews the sample version of Cochran's formula (Cox, 2007) and includes a new result on the robust covariances from the long and short regressions, respectively.

LEMMA B2. *With an $N \times 1$ vector $Y$, an $N \times L_1$ matrix $X_1$, and an $N \times L_2$ matrix $X_2$, fit the following regressions by least squares:*

$$
\begin{aligned}
Y &= X_1\hat{\beta}_1 + X_2\hat{\beta}_2 + \hat{\epsilon}, && \text{(B2)}\\
Y &= X_1\tilde{\beta}_1 + \tilde{\epsilon}, && \text{(B3)}\\
X_2 &= X_1\Phi + R,
\end{aligned}
$$

*where $\hat{\epsilon}, \tilde{\epsilon}$, and $R$ are the residuals. The coefficients satisfy*

$$\tilde{\beta}_1 = \hat{\beta}_1 + \Phi\hat{\beta}_2. \qquad \text{(B4)}$$

*Further let $\hat{V}$ and $\tilde{V}_1$ be the robust covariances of $(\hat{\beta}_1^{\mathrm{T}}, \hat{\beta}_2^{\mathrm{T}})^{\mathrm{T}}$ and $\tilde{\beta}_1$ from* (B2) *and* (B3)*, respectively, and let $\hat{V}_1 = (I, \Phi)\hat{V}(I, \Phi)^{\mathrm{T}}$ be the covariance estimator of $\tilde{\beta}_1$ based on* (B4)*. Then*

$$
\begin{aligned}
\hat{V}_1 &= (X_1^{\mathrm{T}}X_1)^{-1}X_1^{\mathrm{T}}\,\mathrm{diag}(\hat{\epsilon}_i^2)X_1(X_1^{\mathrm{T}}X_1)^{-1},\\
\tilde{V}_1 &= (X_1^{\mathrm{T}}X_1)^{-1}X_1^{\mathrm{T}}\,\mathrm{diag}(\tilde{\epsilon}_i^2)X_1(X_1^{\mathrm{T}}X_1)^{-1}.
\end{aligned}
$$

## B.2. *Definition of the general factorial effects*

Recall that $z_{\mathcal{K}}^* = (z_k^*)_{k\in\mathcal{K}} \in \mathcal{F}_{\mathcal{K}}^*$ indexes the combinations in $\mathcal{F}_{\mathcal{K}} = \prod_{k\in\mathcal{K}}\mathcal{F}_k$ with non-baseline levels in all dimensions. We will also use $q = q_{[K]} = (q_k)_{k=1}^K$ to index a possible treatment combination in $\mathcal{T}$ occasionally when a different letter than $z$ adds clarity. Accordingly, $q_{\mathcal{K}} = (q_k)_{k\in\mathcal{K}} \in \mathcal{F}_{\mathcal{K}}$ and $q_{\overline{\mathcal{K}}} = (q_k)_{k\notin\mathcal{K}} \in \mathcal{F}_{\overline{\mathcal{K}}}$ represent the subvectors of $q$ corresponding to the index sets $\mathcal{K}$ and $\overline{\mathcal{K}}$, respectively. As a special case, let $q_{[m]} = (q_k)_{k=1}^m$ with $\mathcal{K} = [m]$.

Let

$$\mathcal{F}^0(z_{\mathcal{K}}^*) = \{q_{\mathcal{K}} : q_k = z_k^* \text{ or } 0_k \text{ for all } k \in \mathcal{K}\}$$

be the subset of $\mathcal{F}_{\mathcal{K}}$ containing combinations with either $z_k^*$ or $0_k$ in the $k$th dimension for $k \in \mathcal{K}$. For example, the $3 \times 2 \times 2$ factorial experiment has $\mathcal{T} = \{(z_1, z_2, z_3) : z_1 \in \{0_1, 1_1, 2_1\};\ z_2 \in \{0_2, 1_2\};\ z_3 \in \{0_3, 1_3\}\}$, where "$2_1$" denotes the level 2 of factor 1, etc. For $\mathcal{K} = \{1, 2\}$ and $z_{\mathcal{K}}^* = (z_1^*, z_2^*) = (2_1, 1_2)$ as an element in $\mathcal{F}_{\mathcal{K}}^* = \{(1_1, 1_2), (2_1, 1_2)\}$, we have $\mathcal{F}^0(z_{\mathcal{K}}^*) = \{(0_1, 0_2), (0_1, 1_2), (2_1, 0_2), (2_1, 1_2)\}$ featuring factorial combinations $(q_1, q_2)$ of factors in $\mathcal{K}$ with $q_k \in \{0_k, z_k^*\}$.

Let $\bar{Y}(z_{\mathcal{K}}, z_{\overline{\mathcal{K}}}) = \bar{Y}(z)$ be the average potential outcome under $z = (z_{\mathcal{K}}, z_{\overline{\mathcal{K}}}) \in \mathcal{T}$. Lemma B3 gives the explicit forms of the factorial effects in Definitions A1 and A2.

LEMMA B3. *The conditional factorial effects from Definition A*1 *satisfy*

$$\tau(z_{\mathcal{K}}^* \mid z_{\overline{\mathcal{K}}}) = (-1)^{|\mathcal{K}|}\sum_{q_{\mathcal{K}}\in\mathcal{F}_{\mathcal{K}}}\mathcal{I}\{q_{\mathcal{K}} \in \mathcal{F}^0(z_{\mathcal{K}}^*)\}\cdot\mathrm{sgn}(q_{\mathcal{K}})\cdot\bar{Y}(q_{\mathcal{K}}, z_{\overline{\mathcal{K}}}) \qquad \text{(B5)}$$

*for all $z_{\mathcal{K}}^* \in \mathcal{F}_{\mathcal{K}}^*$ and $z_{\overline{\mathcal{K}}} \in \mathcal{F}_{\overline{\mathcal{K}}}$. The general factorial effects from Definition A*2 *satisfy*

$$\tau_\pi(z_{\mathcal{K}}^*) = \sum_{q\in\mathcal{T}}\lambda_q(z_{\mathcal{K}}^*)\cdot\bar{Y}(q)$$

*for all $z_{\mathcal{K}}^* \in \mathcal{F}^*$ with $\lambda_q(z_{\mathcal{K}}^*) = \pi(q_{\overline{\mathcal{K}}})\cdot(-1)^{|\mathcal{K}|}\cdot\mathcal{I}\{q_{\mathcal{K}} \in \mathcal{F}^0(z_{\mathcal{K}}^*)\}\cdot\mathrm{sgn}(q_{\mathcal{K}})$.*

*Proof of Lemma B*3. We first verify (B5) for $\tau(z_{[m]}^* \mid z_{(m+1):K})$ with $\mathcal{K} = [m]$ for all $m = 1, \ldots, K$ by induction. That for general $\tau(z_{\mathcal{K}}^* \mid z_{\overline{\mathcal{K}}})$ then follows by symmetry.

First, direct comparison shows that (B5) holds for $\mathcal{K} = [1]$ at $m = 1$. Assume that (B5) holds for $\mathcal{K} = [m-1]$ with

$$\tau(z_{[m-1]}^* \mid z_{m:K}) = (-1)^{m-1}\sum_{q_{[m-1]}\in\mathcal{F}_{[m-1]}}\mathcal{I}\{q_{[m-1]} \in \mathcal{F}^0(z_{[m-1]}^*)\}\cdot\mathrm{sgn}(q_{[m-1]})\cdot\bar{Y}(q_{[m-1]}, z_{m:K})$$

for all $z^*_{[m-1]} \in \mathcal{F}^*_{[m-1]}$ and $z_{m:K} \in \mathcal{F}_{m:K}$. Then for arbitrary $z^*_{[m]} = (z^*_{[m-1]}, z^*_m) \in \mathcal{F}^*_{[m]}$ and $z_{(m+1):K} \in \mathcal{F}_{(m+1):K}$, we have

$$
\begin{aligned}
&\tau(z^*_{[m]} \mid z_{(m+1):K}) \\
&= \tau(z^*_{[m-1]} \mid z^*_m, z_{(m+1):K}) - \tau(z^*_{[m-1]} \mid 0_m, z_{(m+1):K}) \\
&= (-1)^{m-1} \sum_{q_{[m-1]} \in \mathcal{F}_{[m-1]}} \mathcal{I}\{q_{[m-1]} \in \mathcal{F}^0(z^*_{[m-1]})\} \cdot \operatorname{sgn}(q_{[m-1]}) \cdot \bar{Y}(q_{[m-1]}, z^*_m, z_{(m+1):K}) \\
&\quad - (-1)^{m-1} \sum_{q_{[m-1]} \in \mathcal{F}_{[m-1]}} \mathcal{I}\{q_{[m-1]} \in \mathcal{F}^0(z^*_{[m-1]})\} \cdot \operatorname{sgn}(q_{[m-1]}) \cdot \bar{Y}(q_{[m-1]}, 0_m, z_{(m+1):K}) \\
&= (-1)^{m} \sum_{q_{[m]} \in \mathcal{F}_{[m]}} \mathcal{I}\{q_{[m]} \in \mathcal{F}^0(z^*_{[m]})\} \cdot \operatorname{sgn}(q_{[m]}) \cdot \bar{Y}(q_{[m]}, z_{(m+1):K})
\end{aligned}
$$

such that (B5) holds for $\mathcal{K} = [m]$ as well; the last equality follows from $\|q_{[m]}\|_0 = \|q_{[m-1]}\|_0 + 1$ for $q_{[m]} = (q_{[m-1]}, z^*_m)$ and $\|q_{[m]}\|_0 = \|q_{[m-1]}\|_0$ for $q_{[m]} = (q_{[m-1]}, 0_m)$. This verifies the result for $\tau(z^*_{[m]} \mid z_{(m+1):K})$ for all $m = 1, \ldots, K$ by induction.

We then verify the result for the marginal effects $\tau_\pi(z^*_{\mathcal{K}})$. By (B5),

$$
\tau(z^*_{\mathcal{K}} \mid q_{\overline{\mathcal{K}}}) = \sum_{q_{\mathcal{K}} \in \mathcal{F}_{\mathcal{K}}} \lambda_q(z^*_{\mathcal{K}}) / \pi(q_{\overline{\mathcal{K}}}) \cdot \bar{Y}(q),
$$

where $q = (q_{\mathcal{K}}, q_{\overline{\mathcal{K}}}) \in \mathcal{T}$. Plug this in the definition of $\tau_\pi(z^*_{\mathcal{K}})$ to see

$$
\tau_\pi(z^*_{\mathcal{K}}) = \sum_{q_{\overline{\mathcal{K}}} \in \mathcal{F}_{\overline{\mathcal{K}}}} \pi(q_{\overline{\mathcal{K}}}) \cdot \tau(z^*_{\mathcal{K}} \mid q_{\overline{\mathcal{K}}}) = \sum_{q_{\overline{\mathcal{K}}} \in \mathcal{F}_{\overline{\mathcal{K}}}} \sum_{q_{\mathcal{K}} \in \mathcal{F}_{\mathcal{K}}} \lambda_q(z^*_{\mathcal{K}}) \cdot \bar{Y}(q) = \sum_{q \in \mathcal{T}} \lambda_q(z^*_{\mathcal{K}}) \cdot \bar{Y}(q). \qquad \square
$$

We next verify Theorem A2 with Proposition 5 being a special case.

*Proof of Theorem A2.* Let $0_{\mathcal{K}} = (0_k)_{k \in \mathcal{K}}$ be the value of $z_{\mathcal{K}}$ when $z_k = 0_k$ for all $k \in \mathcal{K}$. With $\tau(z^*_{\mathcal{K}} \mid z_{\overline{\mathcal{K}}}) = 0$ for all $|\mathcal{K}| \geq 3$, we have $\tau_\pi(z^*_{\mathcal{K}}) = 0$ for all $|\mathcal{K}| \geq 3$. It thus suffices to verify the result for the first- and second-order effects, namely, $\tau_\pi(z^*_k) = \tau_{\pi_\times}(z^*_k)$ and $\tau_\pi(z^*_k, z^*_{k'}) = \tau_{\pi_\times}(z^*_k, z^*_{k'})$ for $1 \leq k \neq k' \leq K$. We will verify the results for $\tau_\pi(z^*_1)$ and $\tau_\pi(z^*_1, z^*_2)$ for notational simplicity. Those for general $\tau_\pi(z^*_k)$ and $\tau_\pi(z^*_k, z^*_{k'})$ then follow by symmetry. In the subscripts, we use "$k : k'$" to index the set of $\mathcal{K} = \{k, \ldots, k'\}$ for $1 \leq k \leq k' \leq K$.

Definition A1 defines $\tau(z^*_{\mathcal{K}} \mid z_{\overline{\mathcal{K}}})$ for only $z^*_{\mathcal{K}} \in \mathcal{F}^*_{\mathcal{K}}$ with non-baseline levels in all dimensions. To simplify the presentation, expand the notation to $\tau(z_{\mathcal{K}} \mid z_{\overline{\mathcal{K}}})$ for all $z_{\mathcal{K}} \in \mathcal{F}_{\mathcal{K}}$ with $\tau(z_{\mathcal{K}} \mid z_{\overline{\mathcal{K}}}) = 0$ if any of $z_{\mathcal{K}}$'s elements equals zero.

First, let $\tau(z^*_1, z^*_2 \mid 0_{3:2}, z_{3:K}) = \tau(z^*_1, z^*_2 \mid z_{3:K})$ and $\tau(z^*_1, z^*_2 \mid 0_{3:K}, z_{(K+1):K}) = \tau(z^*_1, z^*_2 \mid 0_{3:K})$. The no three-way interactions condition ensures

$$
\tau(z^*_1, z^*_2 \mid 0_{3:(m-1)}, z_{m:K}) - \tau(z^*_1, z^*_2 \mid 0_{3:m}, z_{(m+1):K}) = 0
$$

for all $m = 3, \ldots, K$. As a result,

$$
\begin{aligned}
\tau(z^*_1, z^*_2 \mid z_{3:K}) &= \tau(z^*_1, z^*_2 \mid z_{3:K}) - \tau(z^*_1, z^*_2 \mid 0_3, z_{4:K}) \\
&\quad + \tau(z^*_1, z^*_2 \mid 0_3, z_{4:K}) - \tau(z^*_1, z^*_2 \mid 0_{3:4}, z_{5:K}) \\
&\quad + \tau(z^*_1, z^*_2 \mid 0_{3:4}, z_{5:K}) - \cdots \\
&= \sum_{m=3}^{K} \left\{ \tau(z^*_1, z^*_2 \mid 0_{3:(m-1)}, z_{m:K}) - \tau(z^*_1, z^*_2 \mid 0_{3:m}, z_{(m+1):K}) \right\} + \tau(z^*_1, z^*_2 \mid 0_{3:K}) \\
&= \tau(z^*_1, z^*_2 \mid 0_{3:K}) \qquad \text{(B6)}
\end{aligned}
$$

are identical over all $z_{3:K} \in \mathcal{F}_{3:K}$ with $\tau_\pi(z^*_1, z^*_2) = \sum_{z_{3:K}} \pi(z_{3:K}) \cdot \tau(z^*_1, z^*_2 \mid z_{3:K}) = \tau(z^*_1, z^*_2 \mid 0_{3:K})$ independent of $\pi$. This ensures $\tau_\pi(z^*_1, z^*_2) = \tau_{\pi_\times}(z^*_1, z^*_2)$ for arbitrary $\pi$.

Second, let $z_{\overline{1m}} = z_{\overline{\{1,m\}}} = (z_k)_{k \notin \{1,m\}}$ and $0_{\overline{1m}} = 0_{\overline{\{1,m\}}} = (0_k)_{k \notin \{1,m\}}$ be the subvectors of $z$ and $0_{[K]}$ without the first and the $m$th elements, respectively, for $m = 2, \ldots, K$; we abbreviate $\overline{\{1,m\}}$ as $\overline{1m}$ in the subscripts when no confusion would arise. Equality (B6) ensures

$$\tau(z_1, z_m \mid z_{\overline{1m}}) = \tau(z_1, z_m \mid 0_{\overline{1m}}) \qquad \text{for all } \ z_1 \in \mathcal{F}_1, z_m \in \mathcal{F}_m, \text{ and } \ z_{\overline{1m}} \in \mathcal{F}_{\overline{1m}}. \tag{B7}$$

Let $\tau(z_1^* \mid 0_{2:1}, z_{2:K}) = \tau(z_1^* \mid z_{2:K})$, $\tau(z_1^* \mid 0_{2:K}, z_{(K+1):K}) = \tau(z_1^* \mid 0_{2:K})$, and $\tau(z_1^*, z_K \mid 0_{2:K-1}, z_{(K+1):K}) = \tau(z_1^*, z_K \mid 0_{2:K-1})$. It follows from (B7) that

$$\tau(z_1^* \mid 0_{2:(m-1)}, z_{m:K}) - \tau(z_1^* \mid 0_{2:m}, z_{(m+1):K}) = \tau(z_1^*, z_m \mid 0_{2:(m-1)}, z_{(m+1):K}) = \tau(z_1^*, z_m \mid 0_{\overline{1m}})$$

for all $m = 2, \ldots, K$ such that

$$\begin{aligned}
\tau(z_1 \mid z_{2:K}) &= \sum_{m=2}^{K} \left\{ \tau(z_1^* \mid 0_{2:(m-1)}, z_{m:K}) - \tau(z_1^* \mid 0_{2:m}, z_{(m+1):K}) \right\} + \tau(z_1^* \mid 0_{2:K}) \\
&= \sum_{m=2}^{K} \tau(z_1^*, z_m \mid 0_{\overline{1m}}) + \tau(z_1^* \mid 0_{2:K}).
\end{aligned}$$

This ensures

$$\begin{aligned}
\tau_\pi(z_1^*) &= \sum_{z_{2:K}} \pi(z_{2:K}) \cdot \tau(z_1^* \mid z_{2:K}) \\
&= \sum_{z_{2:K}} \pi(z_{2:K}) \left\{ \sum_{m=2}^{K} \tau(z_1^*, z_m \mid 0_{\overline{1m}}) \right\} + \sum_{z_{2:K}} \pi(z_{2:K}) \cdot \tau(z_1^* \mid 0_{2:K}) \\
&= \sum_{m=2}^{K} \sum_{z_{2:K}} \pi(z_{2:K}) \cdot \tau(z_1^*, z_m \mid 0_{\overline{1m}}) + \tau(z_1^* \mid 0_{2:K}) \\
&= \sum_{m=2}^{K} \sum_{z_m \in \mathcal{F}_m} \pi(z_m) \cdot \tau(z_1^*, z_m \mid 0_{\overline{1m}}) + \tau(z_1^* \mid 0_{2:K}),
\end{aligned} \tag{B8}$$

where the last equality follows from

$$\sum_{z_{2:K}} \pi(z_{2:K}) \cdot \tau(z_1^*, z_m \mid 0_{\overline{1m}}) = \sum_{z_m} \sum_{z_{\overline{1m}}} \pi(z_{2:K}) \cdot \tau(z_1^*, z_m \mid 0_{\overline{1m}}) = \sum_{z_m} \pi(z_m) \cdot \tau(z_1^*, z_m \mid 0_{\overline{1m}})$$

by $\sum_{z_{\overline{1m}}} \pi(z_{2:K}) = \pi(z_m)$ under coherent $\pi$. Expression (B8) suggests that $\tau_\pi(z_1^*)$ depends only on the marginal weights $\{\pi(z_m) : z_m \in \mathcal{F}_m, \ m = 2, \ldots, K\}$ when $\pi$ is coherent. This verifies $\tau_\pi(z_1^*) = \tau_{\pi_\times}(z_1^*)$ and thus the sufficiency of Condition A1 to ensure $\tau_\pi = \tau_{\pi_\times}$ for all coherent $\pi$.

To see that Condition A1 is also necessary, consider the special case of the $2^3$ experiment with $\tau_{\text{ABC}} \neq 0$. The conditional effects of factor A satisfy $\tau_{\text{A}|\text{B}=0,\text{C}=1} = \tau_{\text{A}|\text{B}=0,\text{C}=0} + \tau_{\text{AC}|\text{B}=0}$, $\tau_{\text{A}|\text{B}=1,\text{C}=0} = \tau_{\text{A}|\text{B}=0,\text{C}=0} + \tau_{\text{AB}|\text{C}=0}$, and $\tau_{\text{A}|\text{B}=1,\text{C}=1} = \tau_{\text{A}|\text{B}=0,\text{C}=0} + \tau_{\text{AB}|\text{C}=0} + \tau_{\text{AC}|\text{B}=0} + \tau_{\text{ABC}}$, respectively, such that

$$\tau_{\pi,\text{A}} = \tau_{\text{A}}(\pi_{\text{BC}}) = \tau_{\text{A}|\text{B}=0,\text{C}=0} + \pi_{\text{C}=1} \cdot \tau_{\text{AC}|\text{B}=0} + \pi_{\text{B}=1} \cdot \tau_{\text{AB}|\text{C}=0} + \pi_{\text{B}=1,\text{C}=1} \cdot \tau_{\text{ABC}}$$

depends on $\pi_{\text{B}=1,\text{C}=1}$ that may not equal $\pi_{\text{B}=1}\pi_{\text{C}=1}$. This implies $\tau_{\pi,\text{A}} = \tau_{\pi_\times,\text{A}}$ does not always hold. □

A reviewer suggested a compact proof of Theorem A2 based on the Kronecker product notation for factorial effects. Following the suggestion, we provide more details below. Recall $\bar{Y}$ as the vector of $\{\bar{Y}(z) : z \in \mathcal{T}\}$ in lexicographical order. Recall that $\pi_{\mathcal{K}} = \{\pi(z_{\mathcal{K}}) : z_{\mathcal{K}} \in \mathcal{F}_{\mathcal{K}}\}$ denotes the weighting vector over $z_{\mathcal{K}} \in \mathcal{F}_{\mathcal{K}}$ for $\mathcal{K} \in \mathcal{P}_K$. Let $\pi_{[K]}$, $\pi_{2:K}$, $\pi_{3:K}$, and $\pi_k$ be the values of $\pi_{\mathcal{K}}$ at $\mathcal{K} = [K], \{2, \ldots, K\}$, $\mathcal{K} = \{3, \ldots, K\}$, and $\mathcal{K} = \{k\}$ where $k \in [K]$, respectively, with elements arranged in lexicographical order of $z_{\mathcal{K}}$. For $\pi$ that is coherent, it follows from Definition A3 and the properties of the Kronecker

product that

$$\pi_{2:K} = (1_{Q_1}^{\mathrm{T}} \otimes I_{Q_2} \otimes \cdots \otimes I_{Q_K})\pi_{[K]}, \qquad \pi_{3:K} = (1_{Q_1}^{\mathrm{T}} \otimes 1_{Q_2}^{\mathrm{T}} \otimes I_{Q_3} \otimes \cdots \otimes I_{Q_K})\pi_{[K]},$$
$$\pi_2 = (1_{Q_1}^{\mathrm{T}} \otimes I_{Q_2} \otimes 1_{Q_3}^{\mathrm{T}} \otimes \cdots \otimes 1_{Q_K}^{\mathrm{T}})\pi_{[K]}; \tag{B9}$$

likewise for $\pi_k$ $(k = 3, \ldots, K)$.

For $k = 1, \ldots, K$, let $C_k = (-1_{Q_k-1}, I_{Q_k-1})$ be the $(Q_k - 1) \times Q_k$ contrast matrix for factor $k$, and define $C_k(0) = 1_{Q_k}^{\mathrm{T}}$ and $C_k(1) = C_k$. Use a binary vector $x = (x_1, \ldots, x_K)^{\mathrm{T}} \in \{0, 1\}^K$ to indicate the presence of the factors in a particular factorial combination, and use

$$C(x) = C_1(x_1) \otimes \cdots \otimes C_K(x_K)$$

to denote all the contrasts for the scaled standard factorial effects of the corresponding factors. Because $C(x)C(x')^{\mathrm{T}} = 0$ for $x \neq x'$ (Mukerjee & Wu, 2007, Theorem 2.2.3), the rows of $C(x)$, for all binary vector $x$ together, form a basis of the $Q$-dimensional Euclidean space. Mukerjee & Wu (2007, Theorem 2.2.1) ensured that $\ell^{\mathrm{T}}\bar{Y}$ is a standard factorial effect for factors in $x$ if and only if $\ell$ is in the row space of $C(x)$. This result, coupled with Condition A1, implies that $C(x)\bar{Y} = 0$ for every $x$ with $\|x\|_1 \geq 3$, so

$$\bar{Y} \text{ lies in the span of the row vectors of } \{C(x) : \|x\|_1 \leq 2\}. \tag{B10}$$

*Proof of Theorem A*2*, version II.* We first prove the result for the main effects. Without loss of generality, consider the main effects of factor 1. Under the coherent weighting $\pi$, they are vectorized lexicographically as $(C_1 \otimes \pi_{2:K}^{\mathrm{T}})\bar{Y}$; under the corresponding product weighting $\pi_\times$, they are vectorized lexicographically as $(C_1 \otimes \pi_2^{\mathrm{T}} \otimes \cdots \otimes \pi_K^{\mathrm{T}})\bar{Y}$. Therefore, we need to show $U_1\bar{Y} = 0$ where

$$U_1 = C_1 \otimes (\pi_{2:K}^{\mathrm{T}} - \pi_2^{\mathrm{T}} \otimes \cdots \otimes \pi_K^{\mathrm{T}}).$$

By (B10), it suffices to show that $U_1 C(x)^{\mathrm{T}} = 0$ if $\|x\|_1 \leq 2$. Consider three cases.

1. $x_1 = 0$. Then $C(x)^{\mathrm{T}} = 1_{Q_1} \otimes \star$ and
$$U_1 C(x)^{\mathrm{T}} = (C_1 \otimes \star)(1_{Q_1} \otimes \star) = (C_1 1_{Q_1}) \otimes \star = 0$$
because $C_1 1_{Q_1} = 0$.
2. $x_1 = 1$ and $x_2 = \cdots = x_K = 0$. Then $C(x)^{\mathrm{T}} = C_1^{\mathrm{T}} \otimes 1_{Q_2} \otimes \cdots \otimes 1_{Q_K}$ and
$$\begin{aligned} U_1 C(x)^{\mathrm{T}} &= \left\{C_1 \otimes (\pi_{2:K}^{\mathrm{T}} - \pi_2^{\mathrm{T}} \otimes \cdots \otimes \pi_K^{\mathrm{T}})\right\}(C_1^{\mathrm{T}} \otimes 1_{Q_2} \otimes \cdots \otimes 1_{Q_K}) \\ &= (C_1 C_1^{\mathrm{T}}) \otimes \left\{\pi_{2:K}^{\mathrm{T}}(1_{Q_2} \otimes \cdots \otimes 1_{Q_K}) - (\pi_2^{\mathrm{T}} 1_{Q_2}) \otimes \cdots \otimes (\pi_K^{\mathrm{T}} 1_{Q_K})\right\} = 0. \end{aligned}$$
3. $x_1 = 1$ and another coordinate of $x$ equals 1. Without loss of generality, assume $x_2 = 1$ and $x_3 = \cdots = x_K = 0$. Then $C(x)^{\mathrm{T}} = C_1^{\mathrm{T}} \otimes C_2^{\mathrm{T}} \otimes 1_{Q_3} \otimes \cdots \otimes 1_{Q_K}$ and
$$\begin{aligned} U_1 C(x)^{\mathrm{T}} &= \left\{C_1 \otimes (\pi_{2:K}^{\mathrm{T}} - \pi_2^{\mathrm{T}} \otimes \cdots \otimes \pi_K^{\mathrm{T}})\right\}(C_1^{\mathrm{T}} \otimes C_2^{\mathrm{T}} \otimes 1_{Q_3} \otimes \cdots \otimes 1_{Q_K}) \\ &= (C_1 C_1^{\mathrm{T}}) \otimes \left\{\pi_{2:K}^{\mathrm{T}}(C_2^{\mathrm{T}} \otimes 1_{Q_3} \otimes \cdots \otimes 1_{Q_K}) - (\pi_2^{\mathrm{T}} C_2^{\mathrm{T}}) \otimes (\pi_3^{\mathrm{T}} 1_{Q_3}) \cdots \otimes (\pi_K^{\mathrm{T}} 1_{Q_K})\right\} \\ &= (C_1 C_1^{\mathrm{T}}) \otimes \left\{\pi_{2:K}^{\mathrm{T}}(C_2^{\mathrm{T}} \otimes 1_{Q_3} \otimes \cdots \otimes 1_{Q_K}) - \pi_2^{\mathrm{T}} C_2^{\mathrm{T}}\right\} \\ &= 0; \end{aligned}$$
the last equality follows from (B9) which ensures
$$\begin{aligned} \pi_{2:K}^{\mathrm{T}}(C_2^{\mathrm{T}} \otimes 1_{Q_3} \otimes \cdots \otimes 1_{Q_K}) &= \pi_{[K]}^{\mathrm{T}}(1_{Q_1} \otimes I_{Q_2} \otimes \cdots \otimes I_{Q_K})(1 \otimes C_2^{\mathrm{T}} \otimes 1_{Q_3} \otimes \cdots \otimes 1_{Q_K}) \\ &= \pi_{[K]}^{\mathrm{T}}(1_{Q_1} \otimes C_2^{\mathrm{T}} \otimes 1_{Q_3} \otimes \cdots \otimes 1_{Q_K}) \\ &= \pi_{[K]}^{\mathrm{T}}(1_{Q_1} \otimes I_{Q_2} \otimes 1_{Q_3} \otimes \cdots \otimes 1_{Q_K})C_2^{\mathrm{T}} = \pi_2^{\mathrm{T}} C_2^{\mathrm{T}}. \end{aligned}$$

We then prove the result for the two-way interactions. Without loss of generality, consider the interactions between factors 1 and 2. Under the coherent weighting $\pi$, they are vectorized lexicographically as $(C_1 \otimes C_2 \otimes \pi_{3:K}^{\mathrm{T}})\bar{Y}$; under the corresponding product weighting $\pi_\times$, they are vectorized lexicographically as $(C_1 \otimes C_2 \otimes \pi_3^{\mathrm{T}} \otimes \cdots \otimes \pi_K^{\mathrm{T}})\bar{Y}$. Therefore, we need to show $U_{12}\bar{Y} = 0$ where

$$U_{12} = C_1 \otimes C_2 \otimes (\pi_{3:K}^{\mathrm{T}} - \pi_3^{\mathrm{T}} \otimes \cdots \otimes \pi_K^{\mathrm{T}}).$$

By (B10), it suffices to show that $U_{12}C(x)^{\mathrm{T}} = 0$ if $\|x\|_1 \leq 2$. Consider two cases.

1. $x_1 = 0$ or $x_2 = 0$. Then $C(x)^{\mathrm{T}} = 1_{Q_1} \otimes 1_{Q_2} \otimes \star$ and

$$U_{12}C(x)^{\mathrm{T}} = (C_1 \otimes C_2 \otimes \star)(1_{Q_1} \otimes 1_{Q_2} \otimes \star) = (C_1 1_{Q_1}) \otimes (C_2 1_{Q_2}) \otimes \star = 0$$

because $C_1 1_{Q_1} = C_2 1_{Q_2} = 0$.

2. $x_1 = x_2 = 1$ and $x_3 = \cdots = x_K = 0$. Then $C(x)^{\mathrm{T}} = C_1^{\mathrm{T}} \otimes C_2^{\mathrm{T}} \otimes 1_{Q_3} \otimes \cdots \otimes 1_{Q_K}$ and

$$\begin{aligned} U_{12}C(x)^{\mathrm{T}} &= \big\{C_1 \otimes C_2 \otimes (\pi_{3:K}^{\mathrm{T}} - \pi_3^{\mathrm{T}} \otimes \cdots \otimes \pi_K^{\mathrm{T}})\big\}(C_1^{\mathrm{T}} \otimes C_2^{\mathrm{T}} \otimes 1_{Q_3} \otimes \cdots \otimes 1_{Q_K}) \\ &= (C_1C_1^{\mathrm{T}}) \otimes (C_2C_2^{\mathrm{T}}) \otimes \big\{\pi_{3:K}^{\mathrm{T}}(1_{Q_3} \otimes \cdots \otimes 1_{Q_K}) - (\pi_3^{\mathrm{T}}1_{Q_3}) \otimes \cdots \otimes (\pi_K^{\mathrm{T}}1_{Q_K})\big\} \\ &= (C_1C_1^{\mathrm{T}}) \otimes (C_2C_2^{\mathrm{T}}) \otimes \{\pi_{3:K}^{\mathrm{T}}(1_{Q_3} \otimes \cdots \otimes 1_{Q_K}) - 1\} \\ &= 0; \end{aligned}$$

the last equality follows from (B9) which ensures

$$\begin{aligned} \pi_{3:K}^{\mathrm{T}}(1_{Q_3} \otimes \cdots \otimes 1_{Q_K}) &= \pi_{[K]}^{\mathrm{T}}(1_{Q_1} \otimes 1_{Q_2} \otimes I_{Q_3} \otimes \cdots \otimes I_{Q_K})(1 \otimes 1 \otimes 1_{Q_3} \otimes \cdots \otimes 1_{Q_K}) \\ &= \pi_{[K]}^{\mathrm{T}}(1_{Q_1} \otimes \cdots \otimes 1_{Q_K}) = 1. \end{aligned}$$

□

### B.3. *Inference from the factor-based regression with the saturated model*

We next verify Theorem A1 that justifies the inference of $\tau$ from the saturated regression (A2). The result implies Proposition 2, Proposition 4, and Theorem 1 in the main text.

Assume fixed location-shift parameters $\delta$ throughout, with $\delta_\times$ as the product weighting scheme in Definition A4. Let $\tau_{\delta_\times} = G_{\delta_\times}\bar{Y}$ be the corresponding $(Q-1)$-vector of general factorial effects with contrast matrix $G_{\delta_\times}$. Recall $F$ as the design matrix of (A2). Let $f_i$ be the concatenation of 1 and $\{f_i(z_{\mathcal{K}}^*) : z_{\mathcal{K}}^* \in \mathcal{F}^*\}$ for unit $i$ to write $F = (f_1, \ldots, f_N)^{\mathrm{T}}$. Let $T = (t_1, \ldots, t_N)^{\mathrm{T}}$ be the design matrix of the treatment-based regression $Y_i \sim \sum_{z\in\mathcal{T}} \mathcal{I}(Z_i = z)$, where $t_i$ is the vector of $\{\mathcal{I}(Z_i = z) : z \in \mathcal{T}\}$ for unit $i$.

*Proof of Theorem A*1. Recall $\hat{\beta}$ as the coefficient vector from the treatment-based regression with $\hat{\beta} = \hat{Y}$. It thus suffices to verify $\hat{\gamma} = G_{\delta_\times}\hat{\beta}$, with a sufficient and necessary condition being

$$t_i = \Gamma^{\mathrm{T}} f_i, \quad T = F\Gamma, \tag{B11}$$

where $\Gamma = (g_0, G_{\delta_\times}^{\mathrm{T}})^{\mathrm{T}}$ is an invertible $Q \times Q$ matrix for some $Q \times 1$ vector $g_0$, by Lemma B1.

Let $\Gamma_{[-1,]}$ be the submatrix of $\Gamma$ without the first row. We proceed to verify (B11) in two steps. We first express each element in $t_i$ into a linear combination of the elements in $f_i$ and thereby give the explicit expressions of the elements in $\Gamma$. That $\Gamma$ is invertible then follows from $T = F\Gamma$ and $T$ is full-column rank given $N_z > 0$. We then verify $\Gamma_{[-1,]} = G_{\delta_\times}$ by showing that $\tau_{\delta_\times} = \Gamma_{[-1,]}\bar{Y}$. To avoid confusion, we use $q = (q_k)_{k=1}^K \in \mathcal{T}$ to index the elements in $t_i$ as $\mathcal{I}(Z_i = q)$, and use $z_{\mathcal{K}}^* = (z_k^*)_{k\in\mathcal{K}} \in \mathcal{F}^*$ to index the non-intercept elements in $f_i$ as $f_i(z_{\mathcal{K}}^*)$.

First, let $\delta_k(0) = 1 - \sum_{s\in\mathcal{F}_k^*} \delta_k(s)$ to extend the definition of $\delta_k(s)$ for $s \in \mathcal{F}_k^*$ to the baseline level 0. It follows from $\mathcal{I}(Z_{ik} = s) = \mathcal{I}_\delta(Z_{ik} = s) + \delta_k(s)$ for $s \in \mathcal{F}_k^*$ that

$$\mathcal{I}(Z_{ik} = 0) = 1 - \sum_{s\in\mathcal{F}_k^*} \mathcal{I}(Z_{ik} = s) = -\sum_{s\in\mathcal{F}_k^*} \mathcal{I}_\delta(Z_{ik} = s) + \delta_k(0).$$

Direct algebra shows

$$\mathcal{I}(Z_i = q) = \prod_{k=1}^{K} \mathcal{I}(Z_{ik} = q_k)$$

$$= \prod_{k:q_k \neq 0} \{\mathcal{I}_\delta(Z_{ik} = q_k) + \delta_k(q_k)\} \cdot \prod_{k:q_k=0} \left\{ - \sum_{s \in \mathcal{F}_k^*} \mathcal{I}_\delta(Z_{ik} = s) + \delta_k(0) \right\} \quad \text{(B12)}$$

$$= \Gamma_q(1) + \sum_{z_\mathcal{K}^* \in \mathcal{F}^*} \Gamma_q(z_\mathcal{K}^*) \cdot f_i(z_\mathcal{K}^*) \quad \text{(B13)}$$

with

$$\Gamma_q(1) = \prod_{k=1}^{K} \delta_k(q_k), \quad \Gamma_q(z_\mathcal{K}^*) = \prod_{k \notin \mathcal{K}} \delta_k(q_k) \cdot (-1)^{|\mathcal{K}|} \cdot \text{sgn}(q_\mathcal{K}) \cdot \prod_{k \in \mathcal{K}, q_k \neq 0} \mathcal{I}(q_k = z_k^*);$$

the explicit form of $\Gamma_q(z_\mathcal{K}^*)$ follows from

$$\prod_{k:q_k \neq 0} \{\mathcal{I}_\delta(Z_{ik} = q_k) + \delta_k(q_k)\} = \prod_{k \in \mathcal{K}, q_k \neq 0} \{\mathcal{I}_\delta(Z_{ik} = q_k) + \delta_k(q_k)\} \cdot \prod_{k \notin \mathcal{K}, q_k \neq 0} \{\mathcal{I}_\delta(Z_{ik} = q_k) + \delta_k(q_k)\},$$

$$\prod_{k:q_k=0} \left\{ - \sum_{s \in \mathcal{F}_k^*} \mathcal{I}_\delta(Z_{ik} = s) + \delta_k(0) \right\} = \prod_{k \in \mathcal{K}, q_k=0} \left\{ - \sum_{s \in \mathcal{F}_k^*} \mathcal{I}_\delta(Z_{ik} = s) + \delta_k(0) \right\} \cdot \prod_{k \notin \mathcal{K}, q_k=0} \left\{ - \sum_{s \in \mathcal{F}_k^*} \mathcal{I}_\delta(Z_{ik} = s) + \delta_k(0) \right\}$$

in (B12) and a direct comparison of the terms in their product that could contribute to $f_i(z_\mathcal{K}^*)$. Equation (B13) ensures $t_i = \Gamma^\text{T} f_i$ with $\Gamma^\text{T}$ being a $Q \times Q$ matrix consisting of $\{\Gamma_q(1), \Gamma_q(z_\mathcal{K}^*) : q \in \mathcal{T}, z_\mathcal{K}^* \in \mathcal{F}^*\}$. In particular, each of the second to $Q$th columns of $\Gamma^\text{T}$ corresponds to one $z_\mathcal{K}^* \in \mathcal{F}^*$ as the concatenation of $\{\Gamma_q(z_\mathcal{K}^*) : q \in \mathcal{T}\}$ in the same order of $q$'s as in $t_i$. This completes the first step.

The second step then follows from

$$\tau_{\delta_\times}(z_\mathcal{K}^*) = \sum_{q \in \mathcal{T}} \Gamma_q(z_\mathcal{K}^*) \cdot \bar{Y}(q) \qquad \text{for all } z_\mathcal{K}^* \in \mathcal{F}^*$$

by Lemma B3 with $\delta_\times(z_{\overline{\mathcal{K}}}) = \prod_{k \notin \mathcal{K}} \delta_k(z_k)$ and $\mathcal{I}\{q_\mathcal{K} \in \mathcal{F}^0(z_\mathcal{K}^*)\} = \prod_{k \in \mathcal{K}, q_k \neq 0} \mathcal{I}(q_k = z_k^*)$. This verifies (B11) and hence $\hat{\gamma} = G_{\delta_\times} \hat{\beta} = G_{\delta_\times} \hat{Y}$.

The result on the robust covariance then follows from the invariance of least squares to non-degenerate linear transformation of the design matrix. □

A reviewer suggested a more compact proof based on the Kronecker product.

*Proof of Theorem A1, version II.* For $i = 1, \ldots, N$ and $k = 1, \ldots, K$, let $t_{ik} = (\mathcal{I}(Z_{ik} = 0), \mathcal{I}(Z_{ik} = 1), \ldots, \mathcal{I}(Z_{ik} = Q_k - 1))^\text{T}$ and $f_{ik} = (1, \mathcal{I}_\delta(Z_{ik} = 1), \ldots, \mathcal{I}_\delta(Z_{ik} = Q_k - 1))^\text{T}$. The properties of the Kronecker product ensure that $t_i = \otimes_{k=1}^K t_{ik}$ and $f_i = \otimes_{k=1}^K f_{ik}$. On the other hand, direct comparison shows that $t_{ik} = W_k f_{ik}$, where

$$W_k = \left(\begin{array}{c|cccc} \delta_k(0) & -1 & -1 & \ldots & -1 \\ \hline \delta_k(1) & 1 & 0 & \ldots & 0 \\ \vdots & \vdots & \vdots & & \vdots \\ \delta_k(Q_k - 1) & 0 & 0 & \ldots & 1 \end{array}\right) = \left(\begin{array}{c|c} \delta_k(0) & -1_{Q_k-1}^\text{T} \\ \hline \delta_k(1) & \\ \vdots & I_{Q_k-1} \\ \delta_k(Q_k - 1) & \end{array}\right)$$

with $\delta_k(0) = 1 - \sum_{z_k=1}^{Q_k-1} \delta_k(z_k)$. This ensures $t_i = W f_i$, where $W = \otimes_{k=1}^{K} W_k$ is nonsingular given $\det(W_k) = 1$ for all $k = 1, \ldots, K$. Direct comparison shows that $W = \Gamma^{\mathrm{T}}$. This verifies (B11) and hence Theorem A1. □

B.4. *Inference from the factor-based regression with unsaturated models*

We next verify the results under the unsaturated specification (A3) with $\mathcal{F}_+$ as the index set of the factorial effects of interest. Let

$$\tau_{\delta_\times,+} = \{\tau_{\delta_\times}(z^*_{\mathcal{K}}) : z^*_{\mathcal{K}} \in \mathcal{F}_+\} = G_{\delta_\times,+}\bar{Y}, \quad \tau_{\delta_\times,-} = \{\tau_{\delta_\times}(z^*_{\mathcal{K}}) : z^*_{\mathcal{K}} \notin \mathcal{F}_+\} = G_{\delta_\times,-}\bar{Y}$$

be the target and nuisance effects in $\tau_{\delta_\times}$, respectively, with $G_{\delta_\times,+}$, and $G_{\delta_\times,-}$ as the contrast matrices. Assume $\Gamma = (g_0, G^{\mathrm{T}}_{\delta_\times})^{\mathrm{T}}$ as defined in (B11) throughout with $T = F\Gamma$.

Let $f_{+,i} = \{1, f_i(z^*_{\mathcal{K}}) : z^*_{\mathcal{K}} \in \mathcal{F}_+\}$ and $f_{-,i} = \{f_i(z^*_{\mathcal{K}}) : z^*_{\mathcal{K}} \notin \mathcal{F}_+\}$ vectorize the regressors included in and excluded from (A3), respectively. Then $F_+ = (f_{+,1}, \ldots, f_{+,N})^{\mathrm{T}}$ gives the $N \times (1 + |\mathcal{F}_+|)$ design matrix of (A3), and $F_- = F \backslash F_+ = (f_{-,1}, \ldots, f_{-,N})^{\mathrm{T}}$ gives the submatrix of $F$ excluded from (A3). The vectors $f_i$, $f_{+,i}$, and $f_{-,i}$ depend only on the value of $Z_i$. Let $f(z)$, $f_+(z)$, and $f_-(z)$ be their respective values if unit $i$ is assigned to treatment $z \in \mathcal{T}$.

Let $\hat{\theta} = (\hat{\mu}, \hat{\gamma}^{\mathrm{T}})^{\mathrm{T}}$ be the coefficient vector from (A2) including the intercept. We have

$$\hat{\theta} = \Gamma\hat{Y} \tag{B14}$$

by (B11) and Lemma B1. Let $\tilde{\theta}_+ = (\tilde{\mu}, \tilde{\gamma}^{\mathrm{T}}_+)^{\mathrm{T}}$ be the $(1 + |\mathcal{F}_+|) \times 1$ coefficient vector from (A3), including the intercept. Let $\hat{\theta}_+ = (\hat{\mu}, \hat{\gamma}^{\mathrm{T}}_+)^{\mathrm{T}}$ be its counterpart from (A2) as a subvector of $\hat{\theta}$. As a convention, we use hat "ˆ" and tilde "˜" to signify estimators from the saturated and unsaturated regressions, respectively.

Assume throughout the subsection

$$G_{\delta_\times} = \begin{pmatrix} G_{\delta_\times,+} \\ G_{\delta_\times,-} \end{pmatrix}, \quad \tau_{\delta_\times} = \begin{pmatrix} \tau_{\delta_\times,+} \\ \tau_{\delta_\times,-} \end{pmatrix}, \quad f_i = \begin{pmatrix} f_{+,i} \\ f_{-,i} \end{pmatrix}, \quad F = (F_+, F_-), \quad \hat{\gamma} = \begin{pmatrix} \hat{\gamma}_+ \\ \hat{\gamma}_- \end{pmatrix}, \quad \hat{\theta} = \begin{pmatrix} \hat{\mu} \\ \hat{\gamma}_+ \\ \hat{\gamma}_- \end{pmatrix}.$$

Recall $\Phi = (F^{\mathrm{T}}_+ F_+)^{-1} F^{\mathrm{T}}_+ F_-$ and $R = F_- - F_+\Phi$ as the coefficient and residual matrices from the column-wise regression of $F_-$ on $F_+$, respectively. We have

$$\Omega = (F^{\mathrm{T}} F)^{-1} = \begin{pmatrix} S_{11} & S_{12} \\ S_{21} & S_{22} \end{pmatrix} \tag{B15}$$

by (B1) with $S_{22} = (R^{\mathrm{T}} R)^{-1}$, $S_{11} = (F^{\mathrm{T}}_+ F_+)^{-1} + \Phi S_{22} \Phi^{\mathrm{T}}$, and $S_{21} = S^{\mathrm{T}}_{12} = -S_{22}\Phi^{\mathrm{T}}$.

Lemma B4 summarizes some useful algebraic facts for proving the main results.

LEMMA B4. *Under the $Q_1 \times \cdots \times Q_K$ experiment,*

(i) $\tilde{\theta}_+ = \hat{\theta}_+ + \Phi\hat{\gamma}_-$ *with $\Phi$ being a deterministic function of $(e_z)_{z\in\mathcal{T}}$;*
(ii) $\Gamma \operatorname{diag}(N_z^{-1})\Gamma^{\mathrm{T}} = \Omega$ *with $(I, \Phi)\Omega(I, \Phi)^{\mathrm{T}} = S_{11} - \Phi S_{22}\Phi^{\mathrm{T}}$;*
(iii) $N^{-1}\sum_{i=1}^{N} h(f_i, f_{-,i}, f_{+,i}) = \sum_{z\in\mathcal{T}} e_z \cdot h(f(z), f_-(z), f_+(z))$ *for arbitrary function $h(\cdot)$ independent of $N$.*

*Proof of Lemma B4.* For statement (i), the linear relation follows from Lemma B2. Further, with $T^{\mathrm{T}} T = \operatorname{diag}(N_z)$ and $F = T\Gamma^{-1}$ from (B11), we have

$$N^{-1} \begin{pmatrix} F^{\mathrm{T}}_+ F_+ & F^{\mathrm{T}}_+ F_- \\ F^{\mathrm{T}}_- F_+ & F^{\mathrm{T}}_- F_- \end{pmatrix} = N^{-1} F^{\mathrm{T}} F = N^{-1}(\Gamma^{-1})^{\mathrm{T}} T^{\mathrm{T}} T \Gamma^{-1} = (\Gamma^{-1})^{\mathrm{T}} \operatorname{diag}(e_z)\Gamma^{-1} \tag{B16}$$

is deterministic in $(e_z)_{z\in\mathcal{T}}$, with $\Phi$ being a function of the two block matrices, $N^{-1}(F^{\mathrm{T}}_+ F_+)$ and $N^{-1}(F^{\mathrm{T}}_+ F_-)$, in the first row.

Statement (ii) follows from $\Gamma \operatorname{diag}(N_z^{-1})\Gamma^{\mathrm{T}} = (F^{\mathrm{T}} F)^{-1} = \Omega$ by (B15) and (B16), with

$$(I, \Phi)\Omega(I, \Phi)^{\mathrm{T}} = (I, \Phi) \begin{pmatrix} S_{11} & S_{12} \\ S_{21} & S_{22} \end{pmatrix} \begin{pmatrix} I \\ \Phi^{\mathrm{T}} \end{pmatrix} = S_{11} - \Phi S_{22}\Phi^{\mathrm{T}}$$

by direct algebra.

Statement (iii) follows from

$$\sum_{i=1}^{N} h(f_i, f_{-,i}, f_{+,i}) = \sum_{z\in\mathcal{T}}\sum_{i:Z_i=z} h(f_i, f_{-,i}, f_{+,i}) = \sum_{z\in\mathcal{T}}\sum_{i:Z_i=z} h(f(z), f_-(z), f_+(z)). \qquad \square$$

*Proof of Theorem A*3. The linear relation follows from Lemma B4(i). We verify below the sufficient conditions for $D\hat{\gamma}_- = 0$.

First, from (B15), direct algebra ensures

$$(F^{\mathrm{T}}F)^{-1}F^{\mathrm{T}} = \begin{pmatrix} S_{11} & S_{12} \\ S_{21} & S_{22} \end{pmatrix} \begin{pmatrix} F_+^{\mathrm{T}} \\ F_-^{\mathrm{T}} \end{pmatrix} = \begin{pmatrix} \star \\ (R^{\mathrm{T}}R)^{-1}R^{\mathrm{T}} \end{pmatrix} \tag{B17}$$

such that $\hat{\gamma}_- = (R^{\mathrm{T}}R)^{-1}R^{\mathrm{T}}Y$. Second, recall $F_{+[,-1]}$ as the submatrix of $F_+$ without the first column. Apply (B17) to $F_+ = (1_N, F_{+[,-1]})$ to see

$$(F_+^{\mathrm{T}}F_+)^{-1}F_+^{\mathrm{T}} = \begin{pmatrix} \star \\ (R_+^{\mathrm{T}}R_+)^{-1}R_+^{\mathrm{T}} \end{pmatrix}, \quad D = (R_+^{\mathrm{T}}R_+)^{-1}R_+^{\mathrm{T}}F_-,$$

where $R_+ = P_N F_{+[,-1]}$ is the $N \times |\mathcal{F}_+|$ residual matrix from the column-wise regression of $F_{+[,-1]}$ on $1_N$. This ensures $D\hat{\gamma}_- = (R_+^{\mathrm{T}}R_+)^{-1}R_+^{\mathrm{T}}F_-(R^{\mathrm{T}}R)^{-1}R^{\mathrm{T}}Y$, and verifies the sufficiency and necessity of $R_+^{\mathrm{T}}F_-(R^{\mathrm{T}}R)^{-1}R^{\mathrm{T}}Y = F_{+[,-1]}^{\mathrm{T}}P_N F_-(R^{\mathrm{T}}R)^{-1}R^{\mathrm{T}}Y = 0$.

The sufficiency of $F_+^{\mathrm{T}}P_N F_- = 0$ then follows from the equivalence between $F_+^{\mathrm{T}}P_N F_- = 0$ and $F_{+[,-1]}^{\mathrm{T}}P_N F_-$ given $1_N^{\mathrm{T}}P_N F_- = 0$.

The sufficiency of $F_+^{\mathrm{T}}F_- = 0$ follows from the definition of $\Phi$. $\square$

*Proof of Corollary A*1 . Let $F(z_{\mathcal{K}}^*)$ be the $N \times 1$ vector of $\{f_i(z_{\mathcal{K}}^*) : i = 1, \dots, N\}$, as the column in $F$ corresponding to $z_{\mathcal{K}}^*$. By the sufficient condition $F_+^{\mathrm{T}}F_- = 0$ in Theorem A3, it suffices to verify

$$\{F(z_{\mathcal{K}}^*)\}^{\mathrm{T}}F(z_{\mathcal{K}'}^*) = 0 \qquad \text{for all } z_{\mathcal{K}}^* \in \mathcal{F}_{\mathcal{K}},\ z_{\mathcal{K}'}^* \in \mathcal{F}_{\mathcal{K}'} \text{ with } \mathcal{K}' \neq \mathcal{K} \tag{B18}$$

under (i)–(iii). Let $f(z_{\mathcal{K}}^* \mid q_{\mathcal{K}})$ be the value of $f_i(z_{\mathcal{K}}^*)$ if $Z_{i,\mathcal{K}} = (Z_{ik})_{k\in\mathcal{K}} = q_{\mathcal{K}} \in \mathcal{F}_{\mathcal{K}}$. Let $Q_{\mathcal{K}} = |\mathcal{F}_{\mathcal{K}}| = \prod_{k\in\mathcal{K}} Q_k$ be the number of combinations in $\mathcal{F}_{\mathcal{K}}$.

For $\mathcal{K}$ and $\mathcal{K}'$ with no overlap, the balanced design ensures that there are $N(Q_{\mathcal{K}}Q_{\mathcal{K}'})^{-1}$ units under each combination of $(q_{\mathcal{K}}, q_{\mathcal{K}'}) \in \mathcal{F}_{\mathcal{K}} \times \mathcal{F}_{\mathcal{K}'}$. We have

$$\begin{aligned}\{F(z_{\mathcal{K}}^*)\}^{\mathrm{T}}F(z_{\mathcal{K}'}^*) = \sum_{i=1}^{N} f_i(z_{\mathcal{K}}^*)f_i(z_{\mathcal{K}'}^*) &= \frac{N}{Q_{\mathcal{K}}Q_{\mathcal{K}'}} \sum_{(q_{\mathcal{K}},q_{\mathcal{K}'})\in\mathcal{F}_{\mathcal{K}}\times\mathcal{F}_{\mathcal{K}'}} f(z_{\mathcal{K}}^* \mid q_{\mathcal{K}})f(z_{\mathcal{K}'}^* \mid q_{\mathcal{K}'}) \\ &= \frac{N}{Q_{\mathcal{K}}Q_{\mathcal{K}'}} \left\{ \sum_{q_{\mathcal{K}}\in\mathcal{F}_{\mathcal{K}}} f(z_{\mathcal{K}}^* \mid q_{\mathcal{K}}) \right\} \left\{ \sum_{q_{\mathcal{K}'}\in\mathcal{F}_{\mathcal{K}'}} f(z_{\mathcal{K}'}^* \mid q_{\mathcal{K}'}) \right\}.\end{aligned} \tag{B19}$$

The sufficient condition (B18) thus holds as long as $\sum_{q_{\mathcal{K}}\in\mathcal{F}_{\mathcal{K}}} f(z_{\mathcal{K}}^* \mid q_{\mathcal{K}}) = 0$ for all $\mathcal{K}$ and $z_{\mathcal{K}}^* \in \mathcal{F}_{\mathcal{K}}$. We verify this below for $\mathcal{K} = [m]$, where $m = 1, \dots, K$. The result for general $\mathcal{K}$ then follows by symmetry.

First, for $\mathcal{K} = [1] = \{1\}$, we have $f(z_1^* \mid q_1) = \mathcal{I}_\delta(q_1 = z_1^*) = \mathcal{I}(q_1 = z_1^*) - \delta_1(z_1^*)$ such that

$$\sum_{q_1\in\mathcal{F}_1} f(z_1^* \mid q_1) = 1 - Q_1\delta_1(z_1^*) = 0 \tag{B20}$$

for all $z_1^* \in \mathcal{F}_1^*$. Second, for $\mathcal{K} = [m]$ and $z_{[m]}^* = (z_1^*, z_{2:m}^*)$ for $m \geq 2$, we have

$$\sum_{q_{[m]} \in \mathcal{F}_{[m]}} f(z_{[m]}^* \mid q_{[m]}) = \sum_{q_{[m]} \in \mathcal{F}_{[m]}} \prod_{k=1}^{m} \mathcal{I}_\delta(q_k = z_k^*) = \sum_{q_1 \in \mathcal{F}_1} \sum_{q_{2:m} \in \mathcal{F}_{2:m}} \prod_{k=1}^{m} \mathcal{I}_\delta(q_k = z_k^*)$$
$$= \left\{ \sum_{q_1 \in \mathcal{F}_1} \mathcal{I}_\delta(q_1 = z_1^*) \right\} \left\{ \sum_{q_{2:m} \in \mathcal{F}_{2:m}} \prod_{k=2}^{m} \mathcal{I}_\delta(q_k = z_k^*) \right\} = 0$$

for all $z_{[m]}^* \in \mathcal{F}_{[m]}^*$, where the last equality follows from (B20).

For $\mathcal{K}$ and $\mathcal{K}'$ that have overlap, let $\mathcal{H} = \mathcal{K} \cap \mathcal{K}'$, $\mathcal{J} = \mathcal{K} \backslash \mathcal{H}$, and $\mathcal{J}' = \mathcal{K}' \backslash \mathcal{H}$ such that $\mathcal{H} \cup \mathcal{J} = \mathcal{K}$, $\mathcal{H} \cup \mathcal{J}' = \mathcal{K}'$, and $\mathcal{J} \cap \mathcal{J}' = \emptyset$. This ensures

$$f(z_{\mathcal{K}}^* \mid q_{\mathcal{K}}) = f(z_{\mathcal{J}}^* \mid q_{\mathcal{J}}) f(z_{\mathcal{H}}^* \mid q_{\mathcal{H}}), \quad f(z_{\mathcal{K}'}^* \mid q_{\mathcal{K}'}) = f(z_{\mathcal{J}'}^* \mid q_{\mathcal{J}'}) f(z_{\mathcal{H}}^* \mid q_{\mathcal{H}})$$

by the definition of $f_i(z_{\mathcal{K}}^*)$. The balanced design further ensures that there are an equal number of $N(Q_{\mathcal{H}} Q_{\mathcal{J}} Q_{\mathcal{J}'})^{-1}$ units under each combination of $(q_{\mathcal{H}}, q_{\mathcal{J}}, q_{\mathcal{J}'}) \in \mathcal{F}_{\mathcal{H}} \times \mathcal{F}_{\mathcal{J}} \times \mathcal{F}_{\mathcal{J}'}$. We have

$$\{F(z_{\mathcal{K}}^*)\}^{\mathrm{T}} F(z_{\mathcal{K}'}^*) = \sum_{i=1}^{N} f_i(z_{\mathcal{K}}^*) f_i(z_{\mathcal{K}'}^*) = \frac{N}{Q_{\mathcal{H}} Q_{\mathcal{J}} Q_{\mathcal{J}'}} \sum_{(q_{\mathcal{H}}, q_{\mathcal{J}}, q_{\mathcal{J}'}) \in \mathcal{F}_{\mathcal{H} \cup \mathcal{J} \cup \mathcal{J}'}} f(z_{\mathcal{K}}^* \mid q_{\mathcal{K}}) f(z_{\mathcal{K}'} \mid q_{\mathcal{K}'})$$
$$= \frac{N}{Q_{\mathcal{H}} Q_{\mathcal{J}} Q_{\mathcal{J}'}} \sum_{q_{\mathcal{H}} \in \mathcal{F}_{\mathcal{H}}} \{f(z_{\mathcal{H}}^* \mid q_{\mathcal{H}})\}^2 \left\{ \sum_{(q_{\mathcal{J}}, q_{\mathcal{J}'}) \in \mathcal{F}_{\mathcal{J}} \times \mathcal{F}_{\mathcal{J}'}} f(z_{\mathcal{J}}^* \mid q_{\mathcal{J}}) f(z_{\mathcal{J}'}^* \mid q_{\mathcal{J}'}) \right\}$$
$$= 0,$$

where the last equality follows from $\sum_{(q_{\mathcal{J}}, q_{\mathcal{J}'}) \in \mathcal{F}_{\mathcal{J}} \times \mathcal{F}_{\mathcal{J}'}} f(z_{\mathcal{J}}^* \mid q_{\mathcal{J}}) f(z_{\mathcal{J}'}^* \mid q_{\mathcal{J}'}) = 0$ by (B19). □

We next verify the asymptotic appropriateness of $\tilde{\gamma}_+$ and $\tilde{\Psi}_+$ under Condition A2.

*Proof of Theorem A*4. The expectation and asymptotic Normality of $\tilde{\gamma}_+$ follow from Theorem A3 and Theorem A1. We verify below the asymptotic conservativeness of $\tilde{\Psi}_+$.

Recall that $\hat{\theta} = (\hat{\theta}_+^{\mathrm{T}}, \hat{\gamma}_-^{\mathrm{T}})^{\mathrm{T}}$ and $\tilde{\theta}_+$ denote the full coefficient vectors from the saturated and unsaturated regressions, respectively, including the intercepts. Let $\tilde{\Psi}'_+$ be the robust covariance of $\tilde{\theta}_+$ from (A3), with $\tilde{\Psi}_+$ as the lower-right $|\mathcal{F}_+| \times |\mathcal{F}_+|$ submatrix. Let $\hat{\Psi}'$ be the robust covariance of $\hat{\theta}$ from (A2), and let $\hat{\Psi}'_+ = (I, \Phi) \hat{\Psi}' (I, \Phi)^{\mathrm{T}}$ be the estimator of $\mathrm{cov}(\tilde{\theta}_+)$ based on Lemma B4(i).

Recall that $\hat{\theta} = \Gamma \hat{Y}$ from (B14). The invariance of least squares to non-degenerate linear transformation of the design matrix ensures that

$$N\{\hat{\Psi}'_+ - \mathrm{cov}(\tilde{\theta}_+)\} = (I, \Phi) \Gamma S \Gamma^{\mathrm{T}} (I, \Phi)^{\mathrm{T}} + o_{\mathrm{p}}(1). \tag{B21}$$

Observe that $\Delta = (I, D) G_{\delta\times} S G_{\delta\times}^{\mathrm{T}} (I, D)^{\mathrm{T}}$ equals the lower-right $|\mathcal{F}_+| \times |\mathcal{F}_+|$ submatrix of $(I, \Phi) \Gamma S \Gamma^{\mathrm{T}} (I, \Phi)^{\mathrm{T}}$. A sufficient condition for $N\{\tilde{\Psi}_+ - \mathrm{cov}(\tilde{\gamma}_+)\} = \Delta + o_{\mathrm{p}}(1)$ is thus

$$N\{\tilde{\Psi}'_+ - \mathrm{cov}(\tilde{\theta}_+)\} = (I, \Phi) \Gamma S \Gamma^{\mathrm{T}} (I, \Phi)^{\mathrm{T}} + o_{\mathrm{p}}(1),$$

which ensures the appropriateness of $\tilde{\Psi}'_+$ after including the intercept. Given (B21), it suffices to verify

$$N(\tilde{\Psi}'_+ - \hat{\Psi}'_+) = o_{\mathrm{p}}(1). \tag{B22}$$

In addition, Lemma B2 ensures that

$$\hat{\Psi}'_+ = (F_+^{\mathrm{T}} F_+)^{-1} F_+^{\mathrm{T}} \,\mathrm{diag}(\hat{\epsilon}_i^2) F_+ (F_+^{\mathrm{T}} F_+)^{-1}, \quad \tilde{\Psi}'_+ = (F_+^{\mathrm{T}} F_+)^{-1} F_+^{\mathrm{T}} \,\mathrm{diag}(\tilde{\epsilon}_i^2) F_+ (F_+^{\mathrm{T}} F_+)^{-1}$$

with $\hat{\epsilon}_i = Y_i - f_i^{\mathrm{T}} \hat{\theta} = Y_i - f_{+,i}^{\mathrm{T}} \hat{\theta}_+ - f_{-,i}^{\mathrm{T}} \hat{\gamma}_-$ and $\tilde{\epsilon}_i = Y_i - f_{+,i}^{\mathrm{T}} \tilde{\theta}_+$. This ensures

$$N(\tilde{\Psi}'_+ - \hat{\Psi}'_+) = \{N^{-1}(F_+^{\mathrm{T}} F_+)\}^{-1} M \{N^{-1}(F_+^{\mathrm{T}} F_+)\}^{-1},$$

where

$$M = N^{-1}F_+^{\mathrm{T}}\{\mathrm{diag}(\tilde{\epsilon}_i^2) - \mathrm{diag}(\hat{\epsilon}_i^2)\}F_+ = N^{-1}\sum_{i=1}^{N}(\tilde{\epsilon}_i^2 - \hat{\epsilon}_i^2)(f_{+,i}f_{+,i}^{\mathrm{T}}). \tag{B23}$$

With $N^{-1}(F_+^{\mathrm{T}}F_+)$ having a finite limit by (B16), the sufficient condition (B22) holds as long as $M = o_{\mathrm{p}}(1)$. We verify below that this is correct.

First, Lemma B4(i) ensures $\tilde{\theta}_+ = \hat{\theta}_+ + \Phi\hat{\gamma}_-$ and thus

$$\tilde{\epsilon}_i - \hat{\epsilon}_i = (Y_i - f_{+,i}^{\mathrm{T}}\tilde{\theta}_+) - (Y_i - f_{+,i}^{\mathrm{T}}\hat{\theta}_+ - f_{-,i}^{\mathrm{T}}\hat{\gamma}_-) = \hat{\gamma}_-^{\mathrm{T}}h_i, \tag{B24}$$

where $h_i = f_{-,i} - \Phi^{\mathrm{T}}f_{+,i}$.

Second, let $\epsilon_i = Y_i - t_i^{\mathrm{T}}\bar{Y} = \sum_{z\in\mathcal{T}}\{Y_i(z) - \bar{Y}(z)\}\cdot\mathcal{I}(Z_i = z)$ be the theoretical residuals corresponding to the treatment-based regression $Y_i \sim t_i$. With $t_i^{\mathrm{T}} = f_i^{\mathrm{T}}\Gamma$ from (B11), we have $\epsilon_i = Y_i - f_i^{\mathrm{T}}\theta$ for $\theta = \Gamma\bar{Y}$, and thus $\hat{\epsilon}_i = Y_i - f_i^{\mathrm{T}}\hat{\theta} = \epsilon_i - f_i^{\mathrm{T}}(\hat{\theta} - \theta)$. This, together with (B24), ensures

$$\tilde{\epsilon}_i^2 - \hat{\epsilon}_i^2 = (\tilde{\epsilon}_i - \hat{\epsilon}_i)(\tilde{\epsilon}_i + \hat{\epsilon}_i) = 2(\hat{\gamma}_-^{\mathrm{T}}h_i)\epsilon_i - 2(\hat{\gamma}_-^{\mathrm{T}}h_i)f_i^{\mathrm{T}}(\hat{\theta} - \theta) + (\hat{\gamma}_-^{\mathrm{T}}h_i)(h_i^{\mathrm{T}}\hat{\gamma}_-).$$

So (B23) evaluates to

$$\begin{aligned}
M &= N^{-1}\sum_{i=1}^{N}(\tilde{\epsilon}_i^2 - \hat{\epsilon}_i^2)(f_{+,i}f_{+,i}^{\mathrm{T}}) \\
&= N^{-1}\sum_{i=1}^{N}\left\{2\hat{\gamma}_-^{\mathrm{T}}h_i(f_{+,i}f_{+,i}^{\mathrm{T}})\epsilon_i - 2\hat{\gamma}_-^{\mathrm{T}}h_i(f_{+,i}f_{+,i}^{\mathrm{T}})f_i^{\mathrm{T}}(\hat{\theta} - \theta) + \hat{\gamma}_-^{\mathrm{T}}h_i(f_{+,i}f_{+,i}^{\mathrm{T}})h_i^{\mathrm{T}}\hat{\gamma}_-\right\} \\
&= 2(I\otimes\hat{\gamma}_-^{\mathrm{T}})\left\{N^{-1}\sum_{i=1}^{N}(I\otimes h_i)(f_{+,i}f_{+,i}^{\mathrm{T}})\epsilon_i\right\} \\
&\quad - 2(I\otimes\hat{\gamma}_-^{\mathrm{T}})\left\{N^{-1}\sum_{i=1}^{N}(I\otimes h_i)(f_{+,i}f_{+,i}^{\mathrm{T}})(I\otimes f_i^{\mathrm{T}})\right\}\{I\otimes(\hat{\theta} - \theta)\} \\
&\quad + (I\otimes\hat{\gamma}_-^{\mathrm{T}})\left\{N^{-1}\sum_{i=1}^{N}(I\otimes h_i)(f_{+,i}f_{+,i}^{\mathrm{T}})(I\otimes h_i^{\mathrm{T}})\right\}(I\otimes\hat{\gamma}_-) \\
&= 2(I\otimes\hat{\gamma}_-^{\mathrm{T}})M_1 - 2(I\otimes\hat{\gamma}_-^{\mathrm{T}})M_2\{I\otimes(\hat{\theta} - \theta)\} + (I\otimes\hat{\gamma}_-^{\mathrm{T}})M_3(I\otimes\hat{\gamma}_-),
\end{aligned} \tag{B25}$$

where $I$ is the $(|\mathcal{F}_+| + 1)\times(|\mathcal{F}_+| + 1)$ identity matrix and

$$M_1 = N^{-1}\sum_{i=1}^{N}(I\otimes h_i)(f_{+,i}f_{+,i}^{\mathrm{T}})\epsilon_i, \qquad M_2 = N^{-1}\sum_{i=1}^{N}(I\otimes h_i)(f_{+,i}f_{+,i}^{\mathrm{T}})(I\otimes f_i^{\mathrm{T}}),$$

$$M_3 = N^{-1}\sum_{i=1}^{N}(I\otimes h_i)(f_{+,i}f_{+,i}^{\mathrm{T}})(I\otimes h_i^{\mathrm{T}}).$$

Lemma B4(iii) ensures that $M_2$ and $M_3$ both have finite limits. This, together with $\hat{\gamma}_- = o_{\mathrm{p}}(1)$ and $\hat{\theta} - \theta = o_{\mathrm{p}}(1)$ by Theorem A1, ensures that $M = o_{\mathrm{p}}(1)$ if $M_1 = o_{\mathrm{p}}(1)$ in (B25). We verify below that this is correct.

Let $\chi_i = (I\otimes h_i)(f_{+,i}f_{+,i}^{\mathrm{T}})\epsilon_i$ with $M_1 = N^{-1}\sum_{i=1}^{N}\chi_i$. Let $\epsilon_i(z) = Y_i(z) - \bar{Y}(z)$ and $h(z) = f_-(z) - \Phi^{\mathrm{T}}f_+(z)$ be the values of $\epsilon_i$ and $h_i$, respectively, if unit $i$ is assigned to treatment $z\in\mathcal{T}$. Then

$$\hat{\chi}(z) = N_z^{-1}\sum_{i:Z_i=z}\chi_i = \{I\otimes h(z)\}\{f_+(z)f_+^{\mathrm{T}}(z)\}\left\{N_z^{-1}\sum_{i:Z_i=z}\epsilon_i(z)\right\} = o_{\mathrm{p}}(1) \qquad (z\in\mathcal{T}) \qquad \square$$

given $N_z^{-1}\sum_{i:Z_i=z}\epsilon_i(z) = \hat{Y}(z) - \bar{Y}(z) = o_{\mathrm{p}}(1)$. This ensures $M_1 = N^{-1}\sum_{i=1}^{N}\chi_i = \sum_{z\in\mathcal{T}}e_z\hat{\chi}(z) = o_{\mathrm{p}}(1)$.

We divide the proof of Theorem A5 into two parts. Part I verifies the bias-variance trade-off and Part II verifies the design-based Gauss–Markov theorem. Recall that $G_{\delta\times,+}$ and $G_{\delta\times,-}$ are the submatrices of $G_{\delta\times}$ that define the factorial effects of interest, $\tau_{\delta\times,+} = G_{\delta\times,+}\bar{Y}$, and the nuisance effects, $\tau_{\delta\times,-} = G_{\delta\times,-}\bar{Y}$, respectively.

*Proof of Theorem A5, Part I.* Condition 2 ensures $S = s_0 J$ with

$$\mathrm{cov}(\hat{Y}) = s_0\{\mathrm{diag}(N_z^{-1}) - N^{-1}J\}. \quad \text{(B26)}$$

From (B14), we have $\tilde{\theta}_+ = (I, \Phi)\hat{\theta} = (I, \Phi)\Gamma\hat{Y}$ with

$$\begin{aligned}
\mathrm{cov}(\tilde{\theta}_+) &= (I, \Phi)\Gamma\mathrm{cov}(\hat{Y})\Gamma^{\mathrm{T}}(I, \Phi)^{\mathrm{T}} \\
&= s_0(I, \Phi)\Gamma\,\mathrm{diag}(N_z^{-1})\Gamma^{\mathrm{T}}(I, \Phi)^{\mathrm{T}} - s_0 N^{-1}(I, \Phi)\Gamma J\Gamma^{\mathrm{T}}(I, \Phi)^{\mathrm{T}} \\
&= s_0 S_{11} - s_0\Phi S_{22}\Phi^{\mathrm{T}} - s_0 N^{-1}(I, \Phi)\Gamma J\Gamma^{\mathrm{T}}(I, \Phi)^{\mathrm{T}} \\
&\le s_0 S_{11} - s_0\Phi S_{22}\Phi^{\mathrm{T}}
\end{aligned}$$

by Lemma B4(i)–(ii). This ensures

$$\mathrm{cov}(\tilde{\gamma}_+) = \{\mathrm{cov}(\tilde{\theta}_+)\}_{[-1,-1]} \le s_0(S_{11})_{[-1,-1]} - s_0 D S_{22} D^{\mathrm{T}}, \quad \text{(B27)}$$

where $(\cdot)_{[-1,-1]}$ indicates the submatrix without the first row and first column.

On the other hand, let $\Gamma_+ = (g_0, G_{\delta\times,+}^{\mathrm{T}})^{\mathrm{T}}$ to write $\Gamma = (\Gamma_+^{\mathrm{T}}, G_{\delta\times,-}^{\mathrm{T}})^{\mathrm{T}}$. Lemma B4(ii) ensures

$$\begin{pmatrix} S_{11} & S_{12} \\ S_{21} & S_{22} \end{pmatrix} = \Gamma\,\mathrm{diag}(N_z^{-1})\Gamma^{\mathrm{T}} = \left(\begin{array}{c|c} \Gamma_+\,\mathrm{diag}(N_z^{-1})\Gamma_+^{\mathrm{T}} & \Gamma_+\,\mathrm{diag}(N_z^{-1})G_{\delta\times,-}^{\mathrm{T}} \\ \hline G_{\delta\times,-}\,\mathrm{diag}(N_z^{-1})\Gamma_+^{\mathrm{T}} & G_{\delta\times,-}\,\mathrm{diag}(N_z^{-1})G_{\delta\times,-}^{\mathrm{T}} \end{array}\right)$$

such that

$$S_{11} = \Gamma_+\,\mathrm{diag}(N_z^{-1})\Gamma_+^{\mathrm{T}} = \left(\begin{array}{c|c} g_0^{\mathrm{T}}\,\mathrm{diag}(N_z^{-1})g_0 & g_0^{\mathrm{T}}\,\mathrm{diag}(N_z^{-1})G_{\delta\times,+}^{\mathrm{T}} \\ \hline G_{\delta\times,+}\,\mathrm{diag}(N_z^{-1})g_0 & G_{\delta\times,+}\,\mathrm{diag}(N_z^{-1})G_{\delta\times,+}^{\mathrm{T}} \end{array}\right)$$

with $(S_{11})_{[-1,-1]} = G_{\delta\times,+}\,\mathrm{diag}(N_z^{-1})G_{\delta\times,+}^{\mathrm{T}}$. This, together with (B26) and $G_{\delta\times,+}JG_{\delta\times,+}^{\mathrm{T}} = 0$, ensures

$$\mathrm{cov}(\hat{\gamma}_+) = \mathrm{cov}(\hat{\tau}_{\delta\times,+}) = G_{\delta\times,+}\mathrm{cov}(\hat{Y})G_{\delta\times,+}^{\mathrm{T}} = s_0 G_{\delta\times,+}\,\mathrm{diag}(N_z^{-1})G_{\delta\times,+}^{\mathrm{T}} = s_0(S_{11})_{[-1,-1]}.$$

Plugging this in (B27) verifies the bias-variance trade-off between $\tilde{\gamma}_+$ and $\hat{\gamma}_+$. □

*Proof of Theorem A5, Part II.* The proof proceeds in two steps, similar to that of the classic Gauss–Markov theorem for least squares estimation with restrictions on parameters.

First, let $\mathcal{L}$ be the set of the $|\mathcal{F}_+| \times Q$ matrices that ensure $E(L\hat{Y}) = \tau_{\delta\times,+}$ under $\tau_{\delta\times,-} = 0$. For $L \in \mathcal{L}$, we have $(L - G_{\delta\times,+})\bar{Y} = 0$ for all $\bar{Y}$ that satisfy $G_{\delta\times,-}\bar{Y} = 0$. This implies $L - G_{\delta\times,+} = L'G_{\delta\times,-}$ for some $|\mathcal{F}_+| \times (Q - 1 - |\mathcal{F}_+|)$ matrix $L'$. Thus,

$$\mathcal{L} = \{L : L = G_{\delta\times,+} + L'G_{\delta\times,-} \text{ for some } |\mathcal{F}_+| \times (Q - 1 - |\mathcal{F}_+|) \text{ matrix } L'\}$$

is a subset of the $|\mathcal{F}_+| \times Q$ contrast matrices.

Second, let $\tilde{G} = (I, D)G_{\delta\times}$ with $\tilde{\gamma}_+ = (I, D)\hat{\gamma} = (I, D)G_{\delta\times}\hat{Y} = \tilde{G}\hat{Y}$. We have $\tilde{G} \in \mathcal{L}$ such that $\tilde{G} = G_{\delta\times,+} + \tilde{L}'G_{\delta\times,-}$ for some $\tilde{L}'$. From (B26), we have $\mathrm{cov}(\tilde{\gamma}_+) = s_0\tilde{G}\,\mathrm{diag}(N_z^{-1})\tilde{G}^{\mathrm{T}}$ and

$$\begin{aligned}
\mathrm{cov}(L\hat{Y}) &= L\mathrm{cov}(\hat{Y})L^{\mathrm{T}} = s_0 L\,\mathrm{diag}(N_z^{-1})L^{\mathrm{T}} \\
&= \mathrm{cov}(\tilde{\gamma}_+) + s_0(L - \tilde{G})\,\mathrm{diag}(N_z^{-1})(L - \tilde{G})^{\mathrm{T}} \\
&\quad + s_0(L - \tilde{G})\,\mathrm{diag}(N_z^{-1})\tilde{G}^{\mathrm{T}} + s_0\tilde{G}\,\mathrm{diag}(N_z^{-1})(L - \tilde{G})^{\mathrm{T}}
\end{aligned}$$

for arbitrary contrast matrix $L$ under Condition 2. It thus suffices to verify

$$(L - \tilde{G})\,\mathrm{diag}(N_z^{-1})\tilde{G}^{\mathrm{T}} = 0 \qquad \text{for all } L \in \mathcal{L}.$$

With $L - \tilde{G} = (L' - \tilde{L}')G_{\delta\times,-}$, a sufficient condition for this is

$$G_{\delta\times,-}\,\mathrm{diag}(N_z^{-1})G_{\delta\times}^{\mathrm{T}}(I, D)^{\mathrm{T}} = 0. \quad \text{(B28)}$$

We verify below that (B28) is correct.

Recall from (B11) that $\Gamma = (g_0, G_{\delta\times}^{\mathrm{T}})^{\mathrm{T}} = (g_0, G_{\delta\times,+}^{\mathrm{T}}, G_{\delta\times,-}^{\mathrm{T}})^{\mathrm{T}}$ such that

$$\Omega = \Gamma\,\mathrm{diag}(N_z^{-1})\Gamma^{\mathrm{T}} = \begin{pmatrix} g_0^{\mathrm{T}} \\ G_{\delta\times,+} \\ G_{\delta\times,-} \end{pmatrix} \mathrm{diag}(N_z^{-1})(g_0, G_{\delta\times}^{\mathrm{T}}) = \begin{pmatrix} \star & \star \\ \star & \star \\ \star & G_{\delta\times,-}\,\mathrm{diag}(N_z^{-1})G_{\delta\times}^{\mathrm{T}} \end{pmatrix}$$

by (B15) and (B16). This, together with

$$(I, \Phi) = \begin{pmatrix} 1 & 0^{\mathrm{T}} & \Phi_{[1,]} \\ 0 & I & D \end{pmatrix} = \begin{pmatrix} 1 & \star \\ 0 & \tilde{D} \end{pmatrix}, \qquad \text{where } \tilde{D} = (I, D),$$

ensures

$$\Omega(I,\Phi)^{\mathrm{T}} = \begin{pmatrix} \star & \star \\ \star & \star \\ \star & G_{\delta\times,-}\,\mathrm{diag}(N_z^{-1})G_{\delta\times}^{\mathrm{T}} \end{pmatrix} \begin{pmatrix} 1 & 0^{\mathrm{T}} \\ \star & \tilde{D}^{\mathrm{T}} \end{pmatrix} = \begin{pmatrix} \star & \star \\ \star & \star \\ \star & G_{\delta\times,-}\,\mathrm{diag}(N_z^{-1})G_{\delta\times}^{\mathrm{T}}\tilde{D}^{\mathrm{T}} \end{pmatrix}.$$

On the other hand, the definitions of $S_{21}$ and $S_{22}$ from (B15) imply

$$\Omega(I,\Phi)^{\mathrm{T}} = \begin{pmatrix} S_{11} & S_{12} \\ S_{21} & S_{22} \end{pmatrix} \begin{pmatrix} I \\ \Phi^{\mathrm{T}} \end{pmatrix} = \begin{pmatrix} \star \\ 0 \end{pmatrix}.$$

This ensures $G_{\delta\times,-}\,\mathrm{diag}(N_z^{-1})G_{\delta\times}^{\mathrm{T}}\tilde{D}^{\mathrm{T}} = 0$ and thus the sufficient condition (B28). $\square$

### B.5. *Weighted least squares*

*Proof of Proposition A*1. We first verify the equivalence of weighted and ordinary least squares under the saturated specification. Recall $F = (f_1, \ldots, f_N)$ as the design matrix of $Y_i \sim 1 + \sum_{z_{\mathcal{K}}^* \in \mathcal{F}^*} f_i(z_{\mathcal{K}}^*) \sim f_i$, with $f(z)$ as the common value of $f_i$ for $i$'s under treatment $z$. Fitting the saturated regression with weights $(w_i)_{i=1}^N$ is to find $\hat{\theta}$ that minimizes

$$\sum_{i=1}^N w_i (Y_i - f_i^{\mathrm{T}}\theta)^2 = \sum_{z \in \mathcal{T}} \left[ w(z) \sum_{i: Z_i = z} \{Y_i - f(z)^{\mathrm{T}}\theta\}^2 \right].$$

This is equivalent to finding $\hat{\mu}(z)$ that minimizes $\sum_{i:Z_i=z}\{Y_i - \mu(z)\}^2$ for each $z \in \mathcal{T}$, and then solving for $\hat{\theta}$. The solution is unique when $N_z > 0$ for all $z \in \mathcal{T}$ such that the weights have no effect on the value of $\hat{\theta}$. This verifies the equivalence of weighted and ordinary least squares under the saturated regression.

For the unsaturated regression with $w(z) \propto e_z^{-1}$, assume without loss of essential generality $w(z) = e_z^{-1}$. Recall $F_+ = (f_{+,1}, \ldots, f_{+,N})^{\mathrm{T}}$ as the design matrix of the unsaturated specification (A3), with $f_+(z)$ as the common value of $f_{+,i}$ for $i$'s under treatment $z$. Let $W = \mathrm{diag}(w_i)_{i=1}^N$ be the weighting matrix with $w_i = w(Z_i) = e_{Z_i}^{-1}$. Let $U$ be the $|\mathcal{T}| \times (1 + |\mathcal{F}_+|)$ matrix with $\{f_+(z) : z \in \mathcal{T}\}$ as the row vectors. The full vector of the weighted least squares coefficients, including the intercept $\tilde{\mu}_{\text{wls}}$, equals

$$\tilde{\theta}_{\text{wls}} = (\tilde{\mu}_{\text{wls}}, \tilde{\gamma}_{\text{wls},+}^{\mathrm{T}})^{\mathrm{T}} = (F_+^{\mathrm{T}} W F_+)^{-1}(F_+^{\mathrm{T}} W Y) = (U^{\mathrm{T}} U)^{-1} U^{\mathrm{T}} \hat{Y}$$

with

$$F_+^{\mathrm{T}} W F_+ = \sum_{i=1}^N w_i f_{+,i} f_{+,i}^{\mathrm{T}} = \sum_{z \in \mathcal{T}} N_z w(z) f_+(z) f_+(z)^{\mathrm{T}} = N \sum_{z \in \mathcal{T}} f_+(z) f_+(z)^{\mathrm{T}} = N U^{\mathrm{T}} U,$$

$$F_+^{\mathrm{T}} W Y = \sum_{i=1}^N w_i f_{+,i} Y_i = \sum_{z \in \mathcal{T}} w(z) f_+(z) N_z \hat{Y}(z) = N \sum_{z \in \mathcal{T}} f_+(z) \hat{Y}(z) = N U^{\mathrm{T}} \hat{Y}.$$

The $\tilde{\theta}_{\text{wls}}$ is thus numerically identical to the ordinary least squares coefficient vector from the aggregate regression $\hat{Y}(z) \sim f_+(z)$ over $z \in \mathcal{T}$ with $U$ as the design matrix. The same reasoning as the proof of Corollary A1 ensures that the coefficients of $f_+(z)$ from the short regression $\hat{Y}(z) \sim f_+(z)$ are identical to those from the long regression $\hat{Y}(z) \sim f(z)$ when (ii) $\delta_k(z_k^*) = Q_k^{-1}$ for all $k = 1, \ldots, K$ and $z_k^* \in \mathcal{F}_k^*$,

and (iii) the elements in $\mathcal{F}^*_{\mathcal{K}}$ are either all included in the unsaturated specification or all excluded. The equivalence between $\tilde{\gamma}_{\text{wls},+}$ and $\hat{\gamma}_+$ then follows from the fact that the non-intercept coefficients of the long regression $\hat{Y}(z) \sim f(z)$ equal $\hat{\gamma}$. □

## C. Special cases and additional results

### C.1. *The $2^2$ factorial experiment*

Propositions 2 and 3 are special cases of Theorems A1 and A3, respectively. We verify below the explicit form of $\tilde{\gamma}_+$ in Proposition 3.

*Proof of Proposition* 3. Lemma B1 ensures that the non-intercept coefficients from (2) equal those from $Y_i \sim 1 + A_i + B_i$. Let $\tilde{\gamma}_+ = (\tilde{\gamma}_{\text{A}}, \tilde{\gamma}_{\text{B}})^{\text{T}}$ denote the non-intercept coefficients from this unshifted specification without introducing new notation. One way to calculate $\tilde{\gamma}_+$ is to use Lemma B2 or Theorem A3. Below we give a direct proof based on Ding (2020, Theorem 5) which was derived using the Frisch–Waugh–Lovell theorem.

Let "prop" denote the sample proportion. Ding (2020, Theorem 5) ensures $\tilde{\gamma}_{\text{A}} = \pi_{\text{B}=0}\hat{\tau}_{\text{A}|\text{B}=0} + \pi_{\text{B}=1}\hat{\tau}_{\text{A}|\text{B}=1}$, where $\pi_{\text{B}=b}$ is proportional to

$$\text{prop}(A_i = 1 \mid B_i = b) \cdot \text{prop}(A_i = 0 \mid B_i = b) \cdot \text{prop}(B_i = b) = \frac{N_{1b}N_{0b}}{N_{1b} + N_{0b}} = (N_{0b}^{-1} + N_{1b}^{-1})^{-1}$$

for $b = 0, 1$ with $\pi_{\text{B}=0} + \pi_{\text{B}=1} = 1$. Direct algebra verifies the formula of $\pi_{\text{B}=b}$; likewise for $\pi_{\text{A}=a}$. □

### C.2. *The $2^3$ factorial experiment*

Propositions 4–6 are special cases of Theorems A1, A2, and A5, respectively. We verify below the explicit form of $\tilde{\gamma}_+$ in Proposition 6 from (4).

Assume fixed $\delta = (\delta_{\text{A}}, \delta_{\text{B}}, \delta_{\text{C}})$ throughout, and let $\mathcal{F}^* = \{\text{A}, \text{B}, \text{C}, \text{AB}, \text{AC}, \text{BC}, \text{ABC}\}$ and $\mathcal{F}_+ = \{\text{A}, \text{B}, \text{C}, \text{AB}, \text{AC}, \text{BC}\} = \mathcal{F}^* \backslash \{\text{ABC}\}$ denote the sets of effects included in the saturated and unsaturated regressions, respectively. We first consider two regressions based on the uncentered $A_i$, $B_i$, and $C_i$ that afford important stepping stones:

$$Y_i \sim 1 + A_i + B_i + C_i + A_iB_i + A_iC_i + B_iC_i, \tag{C1}$$

$$Y_i \sim A_i + A_iB_i + A_iC_i + \sum_{b,c=0,1} \mathcal{I}(B_i = b, C_i = c). \tag{C2}$$

Let $\tilde{\theta} = (\tilde{\mu}, \tilde{\gamma}_+^{\text{T}})^{\text{T}}$ be the $7 \times 1$ coefficient vector from (4) including the intercept, $\tilde{\mu}$. Let $\tilde{\theta}_0 = (\tilde{\mu}_0, \tilde{\gamma}_{0,+}^{\text{T}})^{\text{T}}$ be the $7 \times 1$ coefficient vector from (C1) with intercept $\tilde{\mu}_0$ and $\tilde{\gamma}_{0,+} = (\tilde{\gamma}_{0,f})_{f \in \mathcal{F}_+}$ corresponding to the non-intercept terms. Let $\tilde{\beta}$ be the $7 \times 1$ coefficient vector from (C2) with $\tilde{\beta}_{\text{A}}$, $\tilde{\beta}_{\text{AB}}$, and $\tilde{\beta}_{\text{AC}}$ as the first three elements indicating the coefficients of $A_i$, $A_iB_i$, and $A_iC_i$, respectively. Let

$$P = \left(\begin{array}{c|ccc} I_3 & \begin{array}{ccc} \delta_{\text{B}} & \delta_{\text{C}} & 0 \\ \delta_{\text{A}} & 0 & \delta_{\text{C}} \\ 0 & \delta_{\text{A}} & \delta_{\text{B}} \end{array} \\ \hline 0_{3\times 3} & I_3 \end{array}\right), \quad d = (\delta_{\text{B}}\delta_{\text{C}}, \delta_{\text{A}}\delta_{\text{C}}, \delta_{\text{A}}\delta_{\text{B}}, \delta_{\text{C}}, \delta_{\text{B}}, \delta_{\text{A}})^{\text{T}}, \quad \sigma = \sum_{z \in \mathcal{T}} e_z^{-1},$$

$$\xi = \sigma^{-1}\left(-\sum_a e_{a00}^{-1}, -\sum_b e_{0b0}^{-1}, -\sum_c e_{00c}^{-1}, \sum_{ab} e_{ab0}^{-1}, \sum_{ac} e_{a0c}^{-1}, \sum_{bc} e_{0bc}^{-1}\right)^{\text{T}}$$

to write $D = P\xi - d$. Let

$$\tau_{0,+} = (\tau_{\text{A}|\text{B}=0,\text{C}=0}, \tau_{\text{B}|\text{A}=0,\text{C}=0}, \tau_{\text{C}|\text{A}=0,\text{B}=0}, \tau_{\text{AB}|\text{C}=0}, \tau_{\text{AC}|\text{B}=0}, \tau_{\text{BC}|\text{A}=0})^{\text{T}}$$

be the vector of the first- and second-order conditional effects when the conditioned factors are all at the baseline levels, and let $\hat{\tau}_{0,+}$ be the moment estimator. Lemma C5 expresses $\tilde{\gamma}_+$ in terms of $\hat{\tau}_{0,+}$ and $\hat{\tau}_{\text{ABC}}$.

Lemma C5. *Under the $2^3$ experiment, the estimator from* (4) *satisfies* $\tilde{\gamma}_+ = P\hat{\tau}_{0,+} + P\xi\hat{\tau}_{\text{ABC}}$.

*Proof of Lemma C5.* We verify the result in two steps: first, $\tilde\gamma_+ = P\tilde\gamma_{0,+}$ and second, $\tilde\gamma_{0,+} = \hat\tau_{0,+} + \xi\hat\tau_{\text{ABC}}$.

First, the regressors in (4) and (C1) satisfy

$$\begin{pmatrix} 1 \\ A_i \\ B_i \\ C_i \\ A_iB_i \\ A_iC_i \\ B_iC_i \end{pmatrix} = \left(\begin{array}{c|ccc|ccc} 1 & & 0_3^{\mathrm T} & & & 0_3^{\mathrm T} & \\ \hline \delta_{\text{A}} & 1 & & & & & \\ \delta_{\text{B}} & & 1 & & & 0_{3\times 3} & \\ \delta_{\text{C}} & & & 1 & & & \\ \hline \delta_{\text{A}}\delta_{\text{B}} & \delta_{\text{B}} & \delta_{\text{A}} & 0 & 1 & & \\ \delta_{\text{A}}\delta_{\text{C}} & \delta_{\text{C}} & 0 & \delta_{\text{A}} & & 1 & \\ \delta_{\text{B}}\delta_{\text{C}} & 0 & \delta_{\text{C}} & \delta_{\text{B}} & & & 1 \end{array}\right) \begin{pmatrix} 1 \\ A_i - \delta_{\text{A}} \\ B_i - \delta_{\text{B}} \\ C_i - \delta_{\text{C}} \\ A_iB_i - \delta_{\text{A}}B_i - \delta_{\text{B}}A_i + \delta_{\text{A}}\delta_{\text{B}} \\ A_iC_i - \delta_{\text{C}}A_i - \delta_{\text{A}}C_i + \delta_{\text{A}}\delta_{\text{C}} \\ B_iC_i - \delta_{\text{B}}C_i - \delta_{\text{C}}B_i + \delta_{\text{B}}\delta_{\text{C}} \end{pmatrix} = P_0^{\mathrm T} \begin{pmatrix} 1 \\ A_i' \\ B_i' \\ C_i' \\ A_i'B_i' \\ A_i'C_i' \\ B_i'C_i' \end{pmatrix},$$

where

$$P_0 = \begin{pmatrix} 1 & \star \\ 0_6 & P \end{pmatrix} \qquad \text{with } \star = (\delta_{\text{A}}, \delta_{\text{B}}, \delta_{\text{C}}, \delta_{\text{A}}\delta_{\text{B}}, \delta_{\text{A}}\delta_{\text{C}}, \delta_{\text{B}}\delta_{\text{C}}).$$

This ensures $\tilde\theta = P_0\tilde\theta_0$ by Lemma B1. Removing the first dimension verifies $\tilde\gamma_+ = P\tilde\gamma_{0,+}$.

Second, we verify below the dimensions in $\tilde\gamma_{0,+} = \hat\tau_{0,+} + \xi\hat\tau_{\text{ABC}}$ corresponding to $(\tilde\gamma_{0,\text{A}}, \tilde\gamma_{0,\text{AB}}, \tilde\gamma_{0,\text{AC}})$. The result for $\tilde\gamma_{0,\text{B}}$, $\tilde\gamma_{0,\text{C}}$, and $\tilde\gamma_{0,\text{BC}}$ then follows by symmetry.

To begin with, the regressors in (C1) and (C2) satisfy

$$\left(\begin{array}{c} A_i \\ A_iB_i \\ A_iC_i \\ \hline 1 \\ B_i \\ C_i \\ B_iC_i \end{array}\right) = \begin{pmatrix} I_3 & \\ & H \end{pmatrix} \left(\begin{array}{c} A_i \\ A_iB_i \\ A_iC_i \\ \hline \mathcal{I}(B_i = 0, C_i = 0) \\ \mathcal{I}(B_i = 0, C_i = 1) \\ \mathcal{I}(B_i = 1, C_i = 0) \\ \mathcal{I}(B_i = 1, C_i = 1) \end{array}\right), \qquad \text{where } H = \begin{pmatrix} +1 & +1 & +1 & +1 \\ & & +1 & +1 \\ & +1 & & +1 \\ & & & +1 \end{pmatrix}. \tag{C3}$$

Lemma B1 ensures $\operatorname{diag}(I_3, H^{\mathrm T})\tilde\theta_0 = \tilde\beta$ when the elements in $\tilde\theta_0$ and $\tilde\beta$ are arranged in the same orders as in (C3). Extract the first three dimensions to see $(\tilde\gamma_{0,\text{A}}, \tilde\gamma_{0,\text{AB}}, \tilde\gamma_{0,\text{AC}}) = (\tilde\beta_{\text{A}}, \tilde\beta_{\text{AB}}, \tilde\beta_{\text{AC}})$. This, together with the Frisch–Waugh–Lovell theorem, allows us to compute $(\tilde\gamma_{0,\text{A}}, \tilde\gamma_{0,\text{AB}}, \tilde\gamma_{0,\text{AC}})$ from (C2) in three steps:

(i) Fit $Y_i \sim \sum_{b,c=0,1}\mathcal{I}(B_i = b, C_i = c)$ to obtain residuals $\tilde Y_i$, vectorized as $\tilde Y$.
(ii) Fit $(A_i, A_iB_i, A_iC_i) \sim \sum_{b,c=0,1}\mathcal{I}(B_i = b, C_i = c)$ column-wise to obtain residuals $R_i = (R_{\text{A},i}, R_{\text{AB},i}, R_{\text{AC},i})$, concatenated as $R = (R_1, \ldots, R_N)^{\mathrm T}$.
(iii) Fit $\tilde Y_i \sim R_i$ to obtain $(\tilde\gamma_{0,\text{A}}, \tilde\gamma_{0,\text{AB}}, \tilde\gamma_{0,\text{AC}})^{\mathrm T} = (\tilde\beta_{\text{A}}, \tilde\beta_{\text{AB}}, \tilde\beta_{\text{AC}})^{\mathrm T} = (R^{\mathrm T}R)^{-1}R^{\mathrm T}\tilde Y$.

We proceed to compute $\tilde Y$, $R$, and $(R^{\mathrm T}R)^{-1}R^{\mathrm T}\tilde Y$ one by one.

To simplify the presentation, stratify the units into four groups by $(B_i, C_i) \in \{0,1\}^2$, indexed by $bc$; write $i \in (bc)$ to indicate units in stratum $bc$. Let $N_{bc} = N_{1bc} + N_{0bc}$ and $e_{bc} = N_{bc}/N$ be the number and proportion of units in stratum $bc$, and let $r_{bc} = N_{1bc}/N_{bc} = e_{1bc}/e_{bc}$ be the proportion of units therein with $A_i = 1$. Standard result ensures that the coefficient of $\mathcal{I}(B_i = b, C_i = c)$ from the regression in step (i) equals

$$\hat Y(bc) = N_{bc}^{-1}\sum_{i\in(bc)} Y_i = r_{bc}\hat Y(1bc) + (1 - r_{bc})\hat Y(0bc).$$

For $i \in (bc)$, we have $\tilde Y_i = Y_i - \hat Y(bc)$, and likewise

$$\begin{aligned} &\hat A(bc) = N_{bc}^{-1}\textstyle\sum_{i\in(bc)} A_i = r_{bc}, && R_{\text{A},i} = A_i - \hat A(bc) = A_i - r_{bc}, \\ &\widehat{AB}(bc) = N_{bc}^{-1}\textstyle\sum_{i\in(bc)} A_iB_i = b\cdot\hat A(bc), && R_{\text{AB},i} = A_iB_i - \widehat{AB}(bc) = b\cdot R_{\text{A},i}, \\ &\widehat{AC}(bc) = N_{bc}^{-1}\textstyle\sum_{i\in(bc)} A_iC_i = c\cdot\hat A(bc), && R_{\text{AC},i} = c\cdot R_{\text{A},i}. \end{aligned} \tag{C4}$$

This completes steps (i) and (ii). We next compute $(R^{\mathrm T}R)^{-1}$ and $R^{\mathrm T}\tilde Y$ for step (iii).

First, let $d_{bc} = e_{bc}r_{bc}(1 - r_{bc}) = e_{1bc}e_{0bc}/e_{bc}$. It follows from (C4) that

$$R_{\text{A}}^{\text{T}}R_{\text{A}} = N\sum_{bc} d_{bc}, \quad R_{\text{A}}^{\text{T}}R_{\text{AB}} = N(d_{11} + d_{10}), \quad R_{\text{A}}^{\text{T}}R_{\text{AC}} = N(d_{11} + d_{01}), \quad R_{\text{AB}}^{\text{T}}R_{\text{AC}} = Nd_{11}$$

such that

$$N^{-1}R^{\text{T}}R = \left(\begin{array}{c|c|c} d_{11} + d_{10} + d_{01} + d_{00} & d_{11} + d_{10} & d_{11} + d_{01} \\ d_{11} + d_{10} & d_{11} + d_{10} & d_{11} \\ d_{11} + d_{01} & d_{11} & d_{11} + d_{01} \end{array}\right),$$

$$(N^{-1}R^{\text{T}}R)^{-1} = \{\det(N^{-1}R^{\text{T}}R)\}^{-1}D_1 = (d_{11}d_{10}d_{01}d_{00})^{-1}\sigma^{-1}D_1 \tag{C5}$$

by direct algebra, where

$$D_1 = \left(\begin{array}{c|c|c} d_{11}d_{01} + d_{11}d_{10} + d_{10}d_{01} & -(d_{11} + d_{01})d_{10} & -(d_{11} + d_{10})d_{01} \\ -(d_{11} + d_{01})d_{10} & (d_{11} + d_{01})(d_{10} + d_{00}) & d_{10}d_{01} - d_{11}d_{00} \\ -(d_{11} + d_{10})d_{01} & d_{10}d_{01} - d_{11}d_{00} & (d_{11} + d_{10})(d_{01} + d_{00}) \end{array}\right)$$

is the adjugate matrix of $N^{-1}R^{\text{T}}R$.

Second, similar algebra from (C4) ensures $N^{-1}R^{\text{T}}\tilde{Y} = D_2\kappa_{\text{A}}$, where

$$D_2 = \begin{pmatrix} d_{11} & d_{10} & d_{01} & d_{00} \\ d_{11} & d_{10} & 0 & 0 \\ d_{11} & 0 & d_{01} & 0 \end{pmatrix}, \quad \kappa_{\text{A}} = (\hat{\tau}_{\text{A}|11}, \hat{\tau}_{\text{A}|10}, \hat{\tau}_{\text{A}|01}, \hat{\tau}_{\text{A}|00})^{\text{T}}.$$

This, together with (C5), ensures

$$\begin{aligned}(\tilde{\gamma}_{0,\text{A}}, \tilde{\gamma}_{0,\text{AB}}, \tilde{\gamma}_{0,\text{AC}})^{\text{T}} &= (R^{\text{T}}R)^{-1}R^{\text{T}}\tilde{Y} = (d_{11}d_{10}d_{01}d_{00})^{-1}\sigma^{-1}D_1D_2\kappa_{\text{A}} \\ &= (\hat{\tau}_{\text{A}|\text{B}=0,\text{C}=0}, \hat{\tau}_{\text{AB}|\text{C}=0}, \hat{\tau}_{\text{AC}|\text{B}=0})^{\text{T}} + \xi_{\text{A}}\hat{\tau}_{\text{ABC}},\end{aligned} \tag{C6}$$

where $\xi_{\text{A}} = \sigma^{-1}(-\sum_a e_{a00}^{-1}, \sum_{ab} e_{ab0}^{-1}, \sum_{ac} e_{a0c}^{-1})^{\text{T}}$ is the subvector of $\xi$ corresponding to $\{\text{A}, \text{AB}, \text{AC}\}$; the last equality follows from

$$(d_{11}d_{10}d_{01}d_{00})^{-1}D_1D_2 = \left(\begin{array}{c|c|c|c} -d_{00}^{-1} & d_{00}^{-1} & d_{00}^{-1} & \sigma - d_{00}^{-1} \\ d_{00}^{-1} + d_{10}^{-1} & \sigma - (d_{00}^{-1} + d_{10}^{-1}) & -d_{00}^{-1} - d_{10}^{-1} & -\sigma + (d_{00}^{-1} + d_{10}^{-1}) \\ d_{00}^{-1} + d_{01}^{-1} & -d_{00}^{-1} - d_{01}^{-1} & \sigma - (d_{00}^{-1} + d_{01}^{-1}) & -\sigma + (d_{00}^{-1} + d_{01}^{-1}) \end{array}\right)$$

by $\sum_{bc} d_{bc}^{-1} = \sigma$ and $\tau_{\text{A}|\text{B}=0,\text{C}=1} = \tau_{\text{A}|\text{B}=0,\text{C}=0} + \tau_{\text{AC}|\text{B}=0}$, $\tau_{\text{A}|\text{B}=1,\text{C}=0} = \tau_{\text{A}|\text{B}=0,\text{C}=0} + \tau_{\text{AB}|\text{C}=0}$, $\tau_{\text{A}|\text{B}=1,\text{C}=1} = \tau_{\text{A}|\text{B}=0,\text{C}=0} + \tau_{\text{AB}|\text{C}=0} + \tau_{\text{AC}|\text{B}=0} + \tau_{\text{ABC}}$. This verifies the dimensions for $(\tilde{\gamma}_{0,\text{A}}, \tilde{\gamma}_{0,\text{AB}}, \tilde{\gamma}_{0,\text{AC}})$ in $\tilde{\gamma}_{0,+} = \hat{\tau}_{0,+} + \xi\hat{\tau}_{\text{ABC}}$ and completes the proof. □

*Proof of Proposition* 6. Let $\hat{\tau}_{\delta\times} = (\hat{\tau}_{\delta\times,f})_{f\in\mathcal{F}^*}$ be the moment estimator of $\tau_{\delta\times} = (\tau_{\delta\times,f})_{f\in\mathcal{F}^*}$ under weighting scheme $\delta_\times$. Let $\tilde{\gamma}_f$ and $\hat{\gamma}_f$ be the elements of $\tilde{\gamma}$ and $\hat{\gamma}$ corresponding to the effect of $f \in \mathcal{F}^*$, respectively. Proposition 4 ensures $\hat{\gamma}_f = \hat{\tau}_{\delta\times,f}$ for all $f \in \mathcal{F}^*$ with $\hat{\tau}_{\delta\times,\text{ABC}} = \hat{\tau}_{\text{ABC}}$. This, together with $\tilde{\gamma}_+ = P\hat{\tau}_{0,+} + P\xi\hat{\tau}_{\text{ABC}}$ by Lemma C5 and $D = P\xi - d$ by definition, ensures that it suffices to verify $\hat{\tau}_{\delta\times,+} = P\hat{\tau}_{0,+} + d\hat{\tau}_{\text{ABC}}$, or equivalently, $\tau_{\delta\times,+} - P\tau_{0,+} = d\tau_{\text{ABC}}$. We verify this dimension by dimension.

Denote by $(P\tau_{0,+})_f$ the dimension in $P\tau_{0,+}$ that corresponds to factorial combination $f \in \mathcal{F}_+$. Direct algebra shows

$$\begin{aligned}(P\tau_{0,+})_{\text{A}} &= \tau_{\text{A}|00} + \delta_{\text{B}}\tau_{\text{AB}|\text{C}=0} + \delta_{\text{C}}\tau_{\text{AC}|\text{B}=0} = \tau_{\text{A}|00} + \delta_{\text{B}}(\tau_{\text{A}|10} - \tau_{\text{A}|00}) + \delta_{\text{C}}(\tau_{\text{A}|01} - \tau_{\text{A}|00}) \\ &= (1 - \delta_{\text{B}} - \delta_{\text{C}})\tau_{\text{A}|00} + \delta_{\text{B}}\tau_{\text{A}|10} + \delta_{\text{C}}\tau_{\text{A}|01}. \\ (P\tau_{0,+})_{\text{AB}} &= \tau_{\text{AB}|\text{C}=0}.\end{aligned}$$

Compare this with

$$\begin{aligned}\tau_{\delta\times,\text{A}} &= (1 - \delta_{\text{B}})(1 - \delta_{\text{C}})\tau_{\text{A}|00} + (1 - \delta_{\text{B}})\delta_{\text{C}}\tau_{\text{A}|01} + \delta_{\text{B}}(1 - \delta_{\text{C}})\tau_{\text{A}|10} + \delta_{\text{B}}\delta_{\text{C}}\tau_{\text{A}|11}, \\ \tau_{\delta\times,\text{AB}} &= \delta_{\text{C}}\tau_{\text{AB}|\text{C}=1} + (1 - \delta_{\text{C}})\tau_{\text{AB}|\text{C}=0} = \tau_{\text{AB}|\text{C}=0} + \delta_{\text{C}}\tau_{\text{ABC}}\end{aligned}$$

to see $\tau_{\delta\times,\text{A}} - (P\tau_{0,+})_{\text{A}} = \delta_{\text{B}}\delta_{\text{C}}\tau_{\text{A}|00} - \delta_{\text{B}}\delta_{\text{C}}\tau_{\text{A}|01} - \delta_{\text{B}}\delta_{\text{C}}\tau_{\text{A}|10} + \delta_{\text{B}}\delta_{\text{C}}\tau_{\text{A}|11} = \delta_{\text{B}}\delta_{\text{C}}\tau_{\text{ABC}}$ and $\tau_{\delta\times,\text{AB}} - (P\tau_{0,+})_{\text{AB}} = \delta_{\text{C}}\tau_{\text{ABC}}$. This verifies the result for $\tilde{\gamma}_{\text{A}}$ and $\tilde{\gamma}_{\text{AB}}$. The rest follows by symmetry. □

*Remark* C1. We end this subsection with an example on the average partial effects to illustrate the necessity of product weighting schemes for direct estimation of the general factorial effects when $K \geq 3$. Let $\hat{\gamma}_{0,\text{A}}$, $\hat{\gamma}_{0,\text{B}}$, $\hat{\gamma}_{0,\text{C}}$, $\hat{\gamma}_{0,\text{AB}}$, $\hat{\gamma}_{0,\text{AC}}$, $\hat{\gamma}_{0,\text{BC}}$, and $\hat{\gamma}_{0,\text{ABC}}$ be the non-intercept coefficients from (3) without location shifts. The generalization of strategy (ii) for $2^2$ experiments takes

$$\hat{\gamma}_{\text{e,A},i} = \hat{\gamma}_{0,\text{A}} + \hat{\gamma}_{0,\text{AB}}B_i + \hat{\gamma}_{0,\text{AC}}C_i + \hat{\gamma}_{0,\text{ABC}}B_iC_i$$

to estimate the effect of factor A at the unit level, and computes the average partial effect as

$$\hat{\gamma}_{\text{e,A}} = N^{-1}\sum_{i=1}^{N}\hat{\gamma}_{\text{e,A},i} = \hat{\gamma}_{0,\text{A}} + \hat{\gamma}_{0,\text{AB}}e_{\text{B}=1} + \hat{\gamma}_{0,\text{AC}}e_{\text{C}=1} + \hat{\gamma}_{0,\text{ABC}}e_{\text{B}=1,\text{C}=1}, \tag{C7}$$

where $e_{\text{B}=1} = N^{-1}\sum_{i=1}^{N} B_i$, $e_{\text{C}=1} = N^{-1}\sum_{i=1}^{N} C_i$, and $e_{\text{B}=1,\text{C}=1} = N^{-1}\sum_{i=1}^{N} B_iC_i$. It then follows from $\hat{\gamma}_{0,\text{A}} = \hat{\tau}_{\text{A}|\text{B}=0,\text{C}=0}$,

$$\hat{\gamma}_{0,\text{AB}} = \hat{\tau}_{\text{AB}|\text{C}=0} = \hat{\tau}_{\text{A}|\text{B}=1,\text{C}=0} - \hat{\tau}_{\text{A}|\text{B}=0,\text{C}=0}, \qquad \hat{\gamma}_{0,\text{AC}} = \hat{\tau}_{\text{AC}|\text{B}=0} = \hat{\tau}_{\text{A}|\text{B}=0,\text{C}=1} - \hat{\tau}_{\text{A}|\text{B}=0,\text{C}=0},$$
$$\hat{\gamma}_{0,\text{ABC}} = \hat{\tau}_{\text{ABC}} = \hat{\tau}_{\text{A}|\text{B}=1,\text{C}=1} - \hat{\tau}_{\text{A}|\text{B}=0,\text{C}=1} - \hat{\tau}_{\text{A}|\text{B}=1,\text{C}=0} + \hat{\tau}_{\text{A}|\text{B}=0,\text{C}=0}$$

by Proposition 4 that

$$\hat{\gamma}_{\text{e,A}} = \sum_{b,c} e_{bc}\hat{\tau}_{\text{A}|bc},$$

where $e_{bc} = N^{-1}\sum_{i=1}^{N}\mathcal{I}(B_i = b, C_i = c)$ is the empirical proportion of units with $(B_i, C_i) = (b, c)$ for $b, c = 0, 1$. As a result, when the empirical weighting scheme is not a product weighting scheme, we cannot directly use the coefficient of $A_i'$ to estimate the average partial effect of factor A even after centering, namely $A_i' = A_i - e_{\text{A}=1}$, $B_i' = B_i - e_{\text{B}=1}$, and $C_i' = C_i - e_{\text{C}=1}$ with $e_{\text{A}=1} = N^{-1}\sum_{i=1}^{N} A_i$, unless $\tau_{\text{ABC}} = 0$. In this case, we need to go back to (C7) or the treatment-based regression to compute $\hat{\gamma}_{\text{e,A}}$; likewise for $\hat{\gamma}_{\text{e,B}}$ and $\hat{\gamma}_{\text{e,C}}$. This illustrates the necessity of product weighting schemes for direct estimation of the general factorial effects in the presence of three-way interactions when $K \geq 3$.

### C.3. *The $Q_{\text{A}} \times Q_{\text{B}}$ factorial experiment*

The $Q_{\text{A}} \times Q_{\text{B}}$ experiment features two factors, A and B, of $Q_{\text{A}}$ and $Q_{\text{B}}$ levels, respectively. This gives a total of $Q = Q_{\text{A}}Q_{\text{B}}$ treatment combinations, indexed by $(ab) \in \mathcal{F}_{\text{A}} \times \mathcal{F}_{\text{B}}$ with $\mathcal{F}_{\text{A}} = \{0, \ldots, Q_{\text{A}} - 1\}$ and $\mathcal{F}_{\text{B}} = \{0, \ldots, Q_{\text{B}} - 1\}$. Let $\mathcal{F}_{\text{A}}^* = \mathcal{F}_{\text{A}}\backslash\{0\}$ and $\mathcal{F}_{\text{B}}^* = \mathcal{F}_{\text{B}}\backslash\{0\}$ be the sets of non-baseline levels, indexed by $a^*$ and $b^*$. The regression (A2) simplifies to

$$Y_i \sim 1 + \sum_{a^*\in\mathcal{F}_{\text{A}}^*}\mathcal{I}_\delta(A_i = a^*) + \sum_{b^*\in\mathcal{F}_{\text{B}}^*}\mathcal{I}_\delta(B_i = b^*) + \sum_{a^*\in\mathcal{F}_{\text{A}}^*}\sum_{b^*\in\mathcal{F}_{\text{B}}^*}\mathcal{I}_\delta(A_i = a^*)\mathcal{I}_\delta(B_i = b^*), \tag{C8}$$

where $\mathcal{I}_\delta(A_i = a^*) = \mathcal{I}(A_i = a^*) - \delta_{\text{A}}(a^*)$ and $\mathcal{I}_\delta(B_i = b^*) = \mathcal{I}(B_i = b^*) - \delta_{\text{B}}(b^*)$ with $0 \leq \delta_{\text{A}}(a^*),\ \delta_{\text{B}}(b^*),\ \sum_{a^*\in\mathcal{F}_{\text{A}}^*}\delta_{\text{A}}(a^*),\ \sum_{b^*\in\mathcal{F}_{\text{B}}^*}\delta_{\text{B}}(b^*) \leq 1$.

Let $\hat{\gamma}_{a^*}$, $\hat{\gamma}_{b^*}$, and $\hat{\gamma}_{a^*b^*}$ be the coefficients of $\mathcal{I}_\delta(A_i = a^*)$, $\mathcal{I}_\delta(B_i = b^*)$, and $\mathcal{I}_\delta(A_i = a^*)\mathcal{I}_\delta(B_i = b^*)$ for $a^* \in \mathcal{F}_{\text{A}}^*$ and $b^* \in \mathcal{F}_{\text{B}}^*$ from (C8). Let $\tau(a^* \mid b) = \bar{Y}(a^*b) - \bar{Y}(0b)$, $\tau(b^* \mid a) = \bar{Y}(ab^*) - \bar{Y}(a0)$, and $\tau(a^*b^*) = \bar{Y}(a^*b^*) - \bar{Y}(0b^*) - \bar{Y}(a^*0) + \bar{Y}(00)$ be the conditional main effects and two-way interaction at non-baseline levels $a^*$, $b^*$, and $a^*b^*$, respectively, with $\hat{\tau}(a^* \mid b)$, $\hat{\tau}(b^* \mid a)$, and $\hat{\tau}(a^*b^*)$ as the corresponding moment estimators. As a special case of Theorem A1, we have

$$\hat{\gamma}_{a^*} = \sum_{b\in\mathcal{F}_{\text{B}}}\delta_{\text{B}}(b)\cdot\hat{\tau}(a^* \mid b), \quad \hat{\gamma}_{b^*} = \sum_{a\in\mathcal{F}_{\text{A}}}\delta_{\text{A}}(a)\cdot\hat{\tau}(b^* \mid a), \quad \hat{\gamma}_{a^*b^*} = \hat{\tau}(a^*b^*)$$

with $\delta_{\text{A}}(0) = 1 - \sum_{a^*\in\mathcal{F}_{\text{A}}^*}\delta_{\text{A}}(a^*)$ and $\delta_{\text{B}}(0) = 1 - \sum_{b^*\in\mathcal{F}_{\text{B}}^*}\delta_{\text{B}}(b^*)$. This allows us to infer $\tau_\pi$ under arbitrary $\pi$ from (C8) by setting $\delta_{\text{A}}(a^*) = \pi_{\text{A}=a^*}$ and $\delta_{\text{B}}(b^*) = \pi_{\text{B}=b^*}$ for $a^* \in \mathcal{F}_{\text{A}}^*$ and $b^* \in \mathcal{F}_{\text{B}}^*$. The notion

of product weighting scheme only matters with more than two factors. The properties of the unsaturated variants follow from Theorems A3 and A4.

### C.4. *Comment on the analysis of variance*

The analysis of variance affords another common tool for analyzing factorial experiments, and is closely related to the regression analysis.

Consider the $2^2$ factorial experiment for concreteness. In addition to the running index of $i = 1, \ldots, N$, also denote by "$abr$" the $r$th replicate under treatment combination $(ab) \in \{(00), (01), (10), (11)\}$ for $r = 1, \ldots, N_{ab}$. The analysis of variance model is

$$Y_{abr} = \mu + \alpha_a + \beta_b + \gamma_{ab} + \epsilon_{abr},$$

subject to the zero-sum constraints $\sum_{a=0,1} \alpha_a = 0$, $\sum_{b=0,1} \beta_b = 0$, and $\sum_{a=0,1} \gamma_{ab} = \sum_{b=0,1} \gamma_{ab} = 0$.

Let $\hat{Y} = N^{-1} \sum_{i=1}^{N} Y_i$, $\hat{Y}(a\cdot) = N_{a\cdot}^{-1} \sum_{i:A_i=a} Y_i$, and $\hat{Y}(\cdot b) = N_{\cdot b}^{-1} \sum_{i:B_i=b} Y_i$ be the sample averages over $\{i : i = 1, \ldots, N\}$, $\{i : A_i = a\}$, and $\{i : B_i = b\}$, respectively, with $N_{a\cdot} = Ne_{\text{A}=a}$ and $N_{\cdot b} = Ne_{\text{B}=b}$. Under balanced designs, the moment estimators of the parameters are

$$\hat{\mu} = \hat{Y}, \quad \hat{\alpha}_a = \hat{Y}(a\cdot) - \hat{Y}, \quad \hat{\beta}_b = \hat{Y}(\cdot b) - \hat{Y}, \quad \hat{\gamma}_{ab} = \hat{Y}(ab) - \hat{Y}(a\cdot) - \hat{Y}(\cdot b) + \hat{Y},$$

evaluating to

$$\hat{\alpha}_1 = -\hat{\alpha}_0 = 2^{-1}\hat{\tau}_{\text{A}}(1/2, 1/2), \quad \hat{\beta}_1 = -\hat{\beta}_0 = 2^{-1}\hat{\tau}_{\text{B}}(1/2, 1/2), \quad \hat{\gamma}_{ab} = (-1)^{a+b}4^{-1}\hat{\tau}_{\text{AB}}.$$

The main effects can then be estimated as $\hat{\alpha}_1 - \hat{\alpha}_0 = \hat{\tau}_{\text{A}}(1/2, 1/2)$ and $\hat{\beta}_1 - \hat{\beta}_0 = \hat{\tau}_{\text{B}}(1/2, 1/2)$, respectively, equaling the moment estimators under the equal weighting scheme. This echoes the emphasis by the classic literature to use the analysis of variance specifically for balanced designs. It is equivalent to the least squares fit of $Y_i \sim 1 + A_i^{\text{S}} + B_i^{\text{S}} + A_i^{\text{S}} B_i^{\text{S}}$ under the $\{+1, -1\}$ coding system. Under unbalanced designs, this equivalence breaks down. Fujikoshi (1993) reviewed alternative strategies although they are not commonly used in practice. Nevertheless, the regression analysis can still be used to estimate the standard factorial effects. So we echo Gelman (2005) and view the regression analysis as a general version of the analysis of variance. The above correspondence between the analysis of variance and regression analysis extends to the general $Q_1 \times \cdots \times Q_K$ experiment with minimal modification.

Inference from the analysis of variance, on the other hand, uses $F$-tests based on decompositions of the total sum of squares. However, Ding & Dasgupta (2018) and Wu & Ding (2020) demonstrated that these Normal linear model based tests could lead to incorrect type one error rates under the design-based framework in the presence of heterogeneous treatment effects, and the use of robust standard errors is crucial for the resulting tests to preserve the correct type one error rates. In light of these complications associated with the analysis of variance, we take regression analysis as our final recommendation for analyzing factorial experiments.

### C.5. *Comment on the HC2 robust covariance*

We end this section with a comment on a finite-sample improvement over the robust covariance from the least squares fit, which will be used in the simulation below.

Recall $\hat{V} = \text{diag}\{\hat{S}(z, z)/N_z\}_{z\in\mathcal{T}}$ as a conservative estimator of $\text{cov}(\hat{Y})$. Let $\hat{V}_2$ be the HC2 robust covariance from the treatment-based regression $Y_i \sim \sum_{z\in\mathcal{T}} \mathcal{I}(Z_i = z)$ for a general experiment. We show below that $\hat{V}_2 = \hat{V}$, extending Angrist & Pischke (2009, Chapter 8)'s result on the treatment-control experiment and Lu (2016)'s result on the $2^K$ factorial experiment to the general setting.

Let $T = (t_1, \ldots, t_N)^{\text{T}}$ be the $N \times Q$ design matrix of $Y_i \sim \sum_{z\in\mathcal{T}} \mathcal{I}(Z_i = z)$ with $(T^{\text{T}}T)^{-1} = \text{diag}(N_z^{-1})$. The $i$th diagonal element of $T(T^{\text{T}}T)^{-1}T^{\text{T}}$ equals $t_i^{\text{T}}\,\text{diag}(N_z^{-1})t_i = N_{Z_i}^{-1}$ such that

$$\begin{aligned}\hat{V}_2 &= (T^{\text{T}}T)^{-1}\left[\sum_{i=1}^{N}(1 - N_{Z_i}^{-1})^{-1}\{Y_i - \hat{Y}(Z_i)\}^2 t_i t_i^{\text{T}}\right](T^{\text{T}}T)^{-1} \\ &= \text{diag}(N_z^{-1})\,\text{diag}\{N_z\hat{S}(z, z)\}\,\text{diag}(N_z^{-1}) = \hat{V}.\end{aligned}$$

The result under the saturated factor-based regression (A2) then follows from the invariance of HC2 correction to non-degenerate linear transformation of the design matrix.

## D. NUMERICAL EXAMPLES

### D.1. *Simulation under the $2^4$ factorial experiment*

We now turn to simulation to demonstrate the utility of unsaturated factor-based regressions under the no nuisance effects assumption.

Consider a $2^4$ factorial experiment with $Q = 2^4 = 16$ treatment levels arising from four binary factors, A, B, C, D $\in \{0, 1\}$, and a finite-population $\{Y_i(z) : i = 1, \ldots, N;\ z = 1, \ldots, Q\}$ satisfying the no three-way interactions condition. We consider four regression specifications, one saturated and three unsaturated, for inferring the standard effects under the equal weighting scheme, and evaluate their frequentist operating characteristics under two sample size scenarios, $N_z \in \{2, 3, 4\}$ and $N_z \in \{20, 30, 40\}$ for $z \in \mathcal{T}$, respectively.

Let $A'_i = A_i - 1/2$, $B'_i = B_i - 1/2$, $C'_i = C_i - 1/2$, and $D'_i = D_i - 1/2$ be the location-shifted factor indicators corresponding to the standard factorial effects. The four regressions considered include one saturated regression "rs" with all interactions between $A'_i$, $B'_i$, $C'_i$, and $D'_i$, and three unsaturated regressions, "r1", "r2", and "r3", with up to $m$th-order terms for $m = 1, 2, 3$, respectively:

$$
\begin{aligned}
\text{r1}: \quad & Y_i \sim 1 + A'_i + B'_i + C'_i + D'_i \\
\text{r2}: \quad & Y_i \sim 1 + A'_i + B'_i + C'_i + D'_i + A'_iB'_i + A'_iC'_i + A'_iD'_i + B'_iC'_i + B'_iD'_i + C'_iD'_i \\
\text{r3}: \quad & Y_i \sim 1 + A'_i + B'_i + C'_i + D'_i + A'_iB'_i + A'_iC'_i + A'_iD'_i + B'_iC'_i + B'_iD'_i + C'_iD'_i \\
& \quad + A'_iB'_iC'_i + A'_iB'_iD'_i + A'_iC'_iD'_i + B'_iC'_iD'_i.
\end{aligned}
$$

The no three-way interactions condition on the potential outcomes ensures that regression "r1" is misspecified whereas regressions "r2", "r3", and "rs" are all correct.

Assume that all main effects equal 2, all two-way interactions equal 1, and all three- and four-way interactions equal 0. This determines the $\bar{Y}(z)$'s, which we then use to generate $Y_i(z)$ as $Y_i(z) = \bar{Y}(z) + \epsilon_i(z)$, with $\{\epsilon_i(z)\}_{i=1}^{N-1}$ being independent standard Normals and $\epsilon_N(z) = -\sum_{i=1}^{N-1} \epsilon_i(z)$. For the $Y_i(z)$'s to further satisfy Condition 2, we set $\epsilon_i(z) = \epsilon_i$, with $(\epsilon_i)_{i=1}^{N-1}$ being independent standard Normals and $\epsilon_N = -\sum_{i=1}^{N-1} \epsilon_i$. Fix the potential outcomes in the simulation. We randomly assign the $N$ units to the $Q = 16$ treatment combinations based on the scenario-specific sample sizes, and use the resulting data to form the regressions. We repeat the procedure 1,000 times.

Figure D1 shows the differences between the point estimators and the true parameters for the four main effects under Condition 2; the patterns for the two-way interactions are almost identical and thus omitted. The results are coherent with Theorems A4 and A5 with biased estimators from the misspecified "r1" and increasing variances in the order of "r1" to "rs". Increasing the sample size from $N = 47$ to $N = 470$ reduces the estimation variances yet has no effect on the biases of "r1" due to misspecification. The most parsimonious "r2" shows the smallest sampling variances among all three correct specifications.

Table D1 shows the coverage rates based on the robust covariances and their HC2 corrections discussed in §C.5. For the correctly specified "r2", "r3", and "rs", the classic robust covariances tend to underestimate the variances and thus cause under-coverage when the $N_z$'s are small. Changing to the HC2 covariances or simply increasing the sample size helps alleviate the problem.

### D.2. *More simulation*

We illustrate in this subsection the utility of unsaturated regressions under the large-$Q$-small-$N_z$ scenario. Depending on the size of the study population, the saturated specifications, either treatment-based or factor-based, may sometimes be unfeasible from the outset because of $N < Q$. The asymptotic regime with a diverging $Q$ is challenging and beyond the scope of this paper. We use numeric results to complement our theory, and leave the asymptotic analysis with a diverging $Q$ to future research.

Figure D1. Violin plots of the differences between the estimators and the true parameters for the four main effects.

(i) $N = 47$ with $N_z \in \{2, 3, 4\}$. (ii) $N = 470$ with $N_z \in \{20, 30, 40\}$.

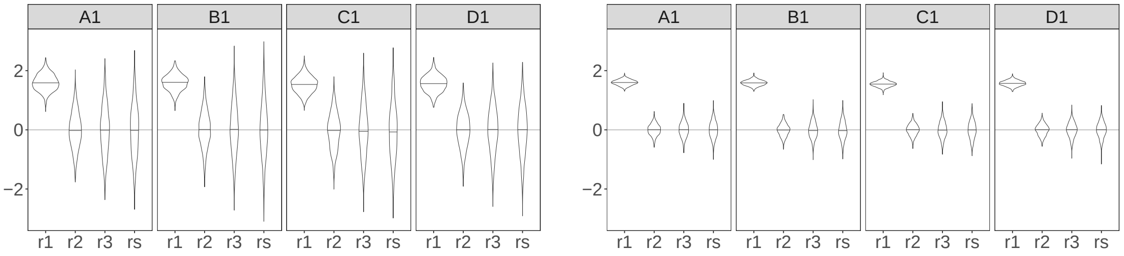


Table D1. *Coverage rates for the main effects over 1,000 replications at the 95% confidence level*

| | | classic robust covariance | | | | HC2 correction | | | |
|---|---|---|---|---|---|---|---|---|---|
| | | A1 | B1 | C1 | D1 | A1 | B1 | C1 | D1 |
| $N = 47$ | r1 | 0.000 | 0.000 | 0.000 | 0.000 | 0.000 | 0.000 | 0.001 | 0.000 |
| | r2 | 0.868 | 0.881 | 0.893 | 0.885 | 0.910 | 0.923 | 0.933 | 0.929 |
| | r3 | 0.792 | 0.783 | 0.788 | 0.815 | 0.880 | 0.869 | 0.889 | 0.878 |
| | rs | 0.754 | 0.704 | 0.710 | 0.763 | 0.837 | 0.803 | 0.821 | 0.844 |
| $N = 470$ | r1 | 0.000 | 0.000 | 0.000 | 0.000 | 0.000 | 0.000 | 0.000 | 0.000 |
| | r2 | 0.946 | 0.942 | 0.952 | 0.945 | 0.949 | 0.945 | 0.959 | 0.949 |
| | r3 | 0.947 | 0.947 | 0.947 | 0.945 | 0.950 | 0.956 | 0.951 | 0.952 |
| | rs | 0.939 | 0.939 | 0.954 | 0.939 | 0.944 | 0.948 | 0.957 | 0.942 |

Assume a $2 \times 3^4$ factorial experiment with $Q = 2 \cdot 3^4 = 162$ treatment combinations arising from one binary factor, A $\in \{0, 1\}$, and four three-level factors, B, C, D, E $\in \{0, 1, 2\}$. We evaluate below the frequentist operating characteristics of regressions "r1", "r2", "r3", and "rs" from §D.1 under two sample-size scenarios as extensions to the asymptotic regime under Condition 1: (i) $N < Q$ with one observation under each of a random set of $N$ distinct treatment combinations; and (ii) $N > Q$ with a random number of two to four units under each treatment combination. Scenario (i) alludes to the setting of fractional factorial designs and defies the use of saturated specifications from the outset. Scenario (ii) guarantees at least $N = 300$ observations in total despite the small $N_z$ under each individual combination, alluding to the large-$Q$ asymptotics of substantial theoretical interest.

Inherit the rest of the settings from §D.1 with "r1" misspecified whereas "r2", "r3", and "rs" all correct. Figure D2 shows the differences between the regression estimators and the true parameters for the nine main effects under Condition 2 over 1,000 replications. The patterns for the two-way interactions are similar and thus omitted.

The result under scenario (ii) accords with the theory and illustrates the utility of factor-based regression even when each $N_z$ is small. The result under scenario (i), on the other hand, further highlights the issue of high variability with complex specifications like "r3" when not all treatment combinations are observed in the study population. Despite both being correctly specified, the more parsimonious "r2" outperforms "r3" markedly in terms of both bias and variance.

Table D2 shows the coverage rates based on the robust covariances with and without the HC2 correction. The over-coverage by the biased "r1" is due to the over-estimation of the standard errors in the presence of biases. For the correctly specified "r2", "r3", and "rs", the robust covariances tend to under-

estimate the variances and thus result in under-coverage when $N_z$'s are small. Changing to the HC2 counterparts or simply increasing the sample size fixes the problem.

A third scenario is when we have exactly one observation under each treatment combination. The point estimators from all four regressions coincide in this case due to the block orthogonality of the full design matrix $F$ under balanced designs; see Corollary A1. The saturated regression, however, defies valid estimation of the standard errors and is thus inapplicable to the Wald-type inference.

### D.3. *Application: hiring discrimination in the United States*

Pedulla (2020) conducted a field experiment examining the hiring discrimination by race, gender, and parental status in the United States. A total of 3,081 job postings were sampled in the 20 largest Metropolitan Statistical Areas under six occupational categories with varying required education levels: administrative assistant, higher-skilled sales, and software developer that often require more education, and cook, customer service, and lower-skilled sales that often require less. A total of 12,324 resumes were then generated, varying along three key dimensions: "race" as signaled by African American or Caucasian sounding names, "gender" as signaled by male or female names, and "parental status" as signaled by listed hobbies that the applicants do with their children or listed volunteer participation in a local Parent Teacher Association. The outcome of interest is whether an applicant received a positive response from the employer. This defines a $2^3$ factorial experiment with occupation as the stratifying covariate. We use the 2,188 observations under the software developer category to illustrate the utility of unsaturated regressions when there is high confidence of no three-way interactions.

To this end, we consider nine regressions as the combination of three location-shift schemes, namely (i) $\delta_k(z_k^*) = 0$ corresponding to the baseline weighting scheme, (ii) $\delta_k(z_k^*) = e_k$ corresponding to the empirical weighting scheme with $e_k$ denoting the empirical treatment proportion of factor $k$, and (iii) $\delta_k(z_k^*) = Q_k^{-1}$ corresponding to the equal weighting scheme, and three specification schemes, namely the saturated specification "rs", the unsaturated specification with up to two-way interactions "r2", and the unsaturated specification with only main effects, "r1".

Table D3 summarizes the results. The three saturated regressions show consistent results of no evidence of two- or three-way interactions. Assume this affords a reasonable representation of the truth. All three specification schemes are thus correct, yielding unbiased point estimators of the factorial effects of interest. Compare across rows of different location-shift schemes. The identicalness of the three location-shift schemes under specification "r1" follows from the invariance of least squares to non-degenerate linear transformation of the design matrix. Compare across columns of different specification schemes. The results under the empirical and equal weighting schemes remain almost unchanged in terms of statistical significance. Those under the baseline weighting scheme, on the other hand, see a gradual increase in the negative effect of being an African American. The standard errors show a clear decreasing trend as the specifications become more parsimonious under the baseline and equal weighting schemes, illustrating the gain in efficiency with the simpler specifications.

Overall, having an African American-sounding name significantly decreases the probability of getting a positive response for software developer jobs.

Figure D2. Violin plots of the differences between the point estimators and the true parameters over 1,000 replications for the nine main effects under Condition 2. “k1” and “k2” indicate the main effects of factor $k$ at non-baseline levels 1 and 2, respectively, for $k$ = A, B, C, D, E.

(i) $N$ = 100 with one unit under each of the 100 randomly selected treatment combinations.

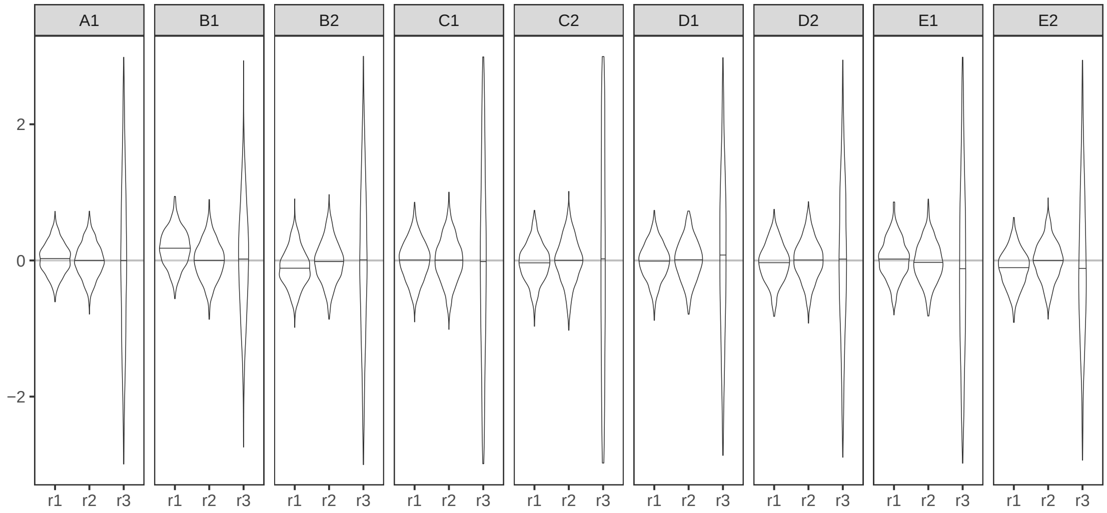


(ii) $N$ = 486 with a random number of two to four units under each treatment combination.

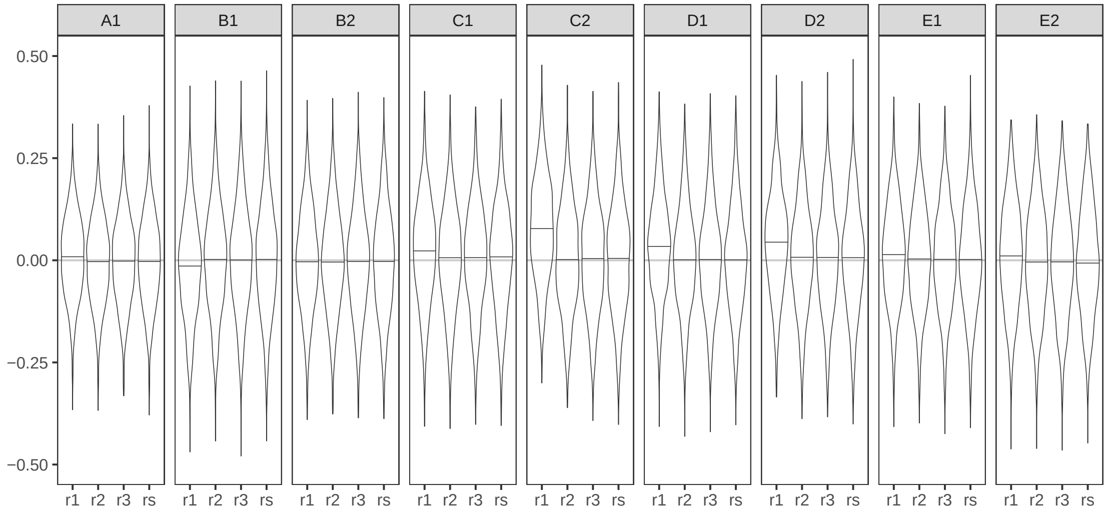

Table D2. *Coverage rates for the nine main effects over 1,000 replications at the 95% confidence level. The HC2 correction is inapplicable to specifications "r3" and "rs" since some leverage scores equal 1*

classic robust covariance

| $N$ | | A1 | B1 | B2 | C1 | C2 | D1 | D2 | E1 | E2 |
|---|---|---|---|---|---|---|---|---|---|---|
| 100 | r1 | 0.981 | 0.946 | 0.965 | 0.982 | 0.984 | 0.983 | 0.973 | 0.979 | 0.952 |
| | r2 | 0.860 | 0.862 | 0.832 | 0.843 | 0.846 | 0.851 | 0.854 | 0.860 | 0.856 |
| | r3 | 0.176 | 0.182 | 0.172 | 0.191 | 0.208 | 0.181 | 0.201 | 0.205 | 0.195 |
| | rs | 0.000 | 0.000 | 0.000 | 0.000 | 0.000 | 0.000 | 0.000 | 0.000 | 0.000 |
| 486 | r1 | 0.979 | 0.983 | 0.985 | 0.977 | 0.957 | 0.977 | 0.977 | 0.982 | 0.983 |
| | r2 | 0.947 | 0.933 | 0.944 | 0.937 | 0.944 | 0.937 | 0.937 | 0.952 | 0.940 |
| | r3 | 0.922 | 0.909 | 0.925 | 0.918 | 0.917 | 0.916 | 0.907 | 0.926 | 0.909 |
| | rs | 0.880 | 0.868 | 0.864 | 0.878 | 0.871 | 0.869 | 0.872 | 0.885 | 0.854 |

HC2 correction

| | | A1 | B1 | B2 | C1 | C2 | D1 | D2 | E1 | E2 |
|---|---|---|---|---|---|---|---|---|---|---|
| 100 | r1 | 0.985 | 0.958 | 0.974 | 0.986 | 0.988 | 0.986 | 0.980 | 0.986 | 0.965 |
| | r2 | 0.956 | 0.955 | 0.945 | 0.947 | 0.938 | 0.949 | 0.952 | 0.938 | 0.941 |
| | r3 | n.a. | n.a. | n.a. | n.a. | n.a. | n.a. | n.a. | n.a. | n.a. |
| | rs | n.a. | n.a. | n.a. | n.a. | n.a. | n.a. | n.a. | n.a. | n.a. |
| 486 | r1 | 0.980 | 0.985 | 0.988 | 0.977 | 0.959 | 0.979 | 0.979 | 0.984 | 0.985 |
| | r2 | 0.958 | 0.952 | 0.954 | 0.950 | 0.952 | 0.953 | 0.948 | 0.959 | 0.948 |
| | r3 | 0.958 | 0.952 | 0.957 | 0.952 | 0.950 | 0.949 | 0.948 | 0.951 | 0.953 |
| | rs | 0.955 | 0.942 | 0.952 | 0.955 | 0.946 | 0.950 | 0.944 | 0.951 | 0.951 |

Table D3. *Stratified analysis of job postings for software developers. Let $\delta = \delta_k(z_k^*)$ indicate the location-shift schemes. (b, w, p) = (black, women, parent). "rs" = saturated regression; "r2" = unsaturated regression with main effects and two-way interactions; "r1" = unsaturated regression with only main effects. Columns "est." report the point estimators, columns "s.e." report the robust standard errors, and columns "p" report the $p$-values from large-sample approximations of the robust $t$-statistics with significance codes 0 '***' 0.001 '**' 0.01 '*' 0.05 '.' 0.1 ' ' 1*

| | | rs | | | r2 | | | r1 | | |
|---|---|---|---|---|---|---|---|---|---|---|
| $\delta$ | | est. | s.e. | $p$ | est. | s.e. | $p$ | est. | s.e. | $p$ |
| 0 | b | -0.016 | 0.019 | 0.414 | -0.018 | 0.015 | 0.24 | -0.026 | 0.013 | 0.043 * |
| | w | 0.018 | 0.02 | 0.375 | 0.016 | 0.015 | 0.296 | 0.004 | 0.013 | 0.741 |
| | p | 0.069 | 0.042 | 0.1 | 0.062 | 0.033 | 0.064 . | 0.025 | 0.018 | 0.183 |
| | b:w | -0.012 | 0.028 | 0.655 | -0.008 | 0.021 | 0.715 | | | |
| | b:p | -0.042 | 0.055 | 0.448 | -0.027 | 0.031 | 0.376 | | | |
| | w:p | -0.062 | 0.055 | 0.263 | -0.048 | 0.032 | 0.129 | | | |
| | b:w:p | 0.029 | 0.074 | 0.692 | | | | | | |
| $e_k$ | b | -0.026 | 0.013 | 0.041 * | -0.026 | 0.012 | 0.031 * | -0.026 | 0.013 | 0.043 * |
| | w | 0.004 | 0.013 | 0.747 | 0.004 | 0.011 | 0.716 | 0.004 | 0.013 | 0.741 |
| | p | 0.025 | 0.018 | 0.179 | 0.024 | 0.02 | 0.225 | 0.025 | 0.018 | 0.183 |
| | b:w | -0.008 | 0.026 | 0.771 | -0.008 | 0.021 | 0.715 | | | |
| | b:p | -0.027 | 0.037 | 0.461 | -0.027 | 0.031 | 0.376 | | | |
| | w:p | -0.047 | 0.037 | 0.199 | -0.048 | 0.032 | 0.129 | | | |
| | b:w:p | 0.029 | 0.074 | 0.692 | | | | | | |
| $1/2$ | b | -0.035 | 0.018 | 0.054 . | -0.035 | 0.018 | 0.056 . | -0.026 | 0.013 | 0.043 * |
| | w | -0.012 | 0.018 | 0.529 | -0.012 | 0.018 | 0.5 | 0.004 | 0.013 | 0.741 |
| | p | 0.025 | 0.018 | 0.179 | 0.024 | 0.02 | 0.226 | 0.025 | 0.018 | 0.183 |
| | b:w | 0.002 | 0.037 | 0.953 | -0.008 | 0.021 | 0.715 | | | |
| | b:p | -0.027 | 0.037 | 0.46 | -0.027 | 0.031 | 0.376 | | | |
| | w:p | -0.047 | 0.037 | 0.201 | -0.048 | 0.032 | 0.129 | | | |
| | b:w:p | 0.029 | 0.074 | 0.692 | | | | | | |

## Bibliography


Angrist, J. D. & Pischke, J.-S. (2009). *Mostly Harmless Econometrics.* Princeton: Princeton University Press.

Cox, D. R. (2007). On a generalization of a result of W. G. Cochran. *Biometrika* **94**, 755–759.

Ding, P. (2020). The Frisch–Waugh–Lovell theorem for standard errors. *Statistics and Probability Letters* **168**, 108945.

Ding, P. & Dasgupta, T. (2018). A randomization-based perspective of analysis of variance: a test statistic robust to treatment effect heterogeneity. *Biometrika* **105**, 45–56.

Fujikoshi, Y. (1993). Two-way ANOVA models with unbalanced data. *Discrete Mathematics* **116**, 315–334.

Gelman, A. (2005). Analysis of variance—why it is more important than ever. *The Annals of Statistics* **33**, 1 – 53.

Lu, J. (2016). On randomization-based and regression-based inferences for $2^K$ factorial designs. *Statistics and Probability Letters* **112**, 72–78.

Mukerjee, R. & Wu, C. F. J. (2007). *A Modern Theory of Factorial Design.* New York: Springer.

Pedulla, D. (2020). A field experiment of race, gender, and parental status discrimination in the United States. Tech. rep., Harvard Dataverse, https://doi.org/10.7910/DVN/4TTCEY.

Wu, J. & Ding, P. (2020). Randomization tests for weak null hypotheses in randomized experiments. *Journal of the American Statistical Association* , https://doi.org/10.1080/01621459.2020.1750415.
